# Supplementary material for: The POlarised GLEAM Survey (POGS) II: Results from an All-Sky Rotation Measure Synthesis Survey at Long Wavelengths
Source: arXiv:2005.09266 ancillary file (2020-11-12)
Supplement: Supplementary file 1 [file Appendix-A.pdf]

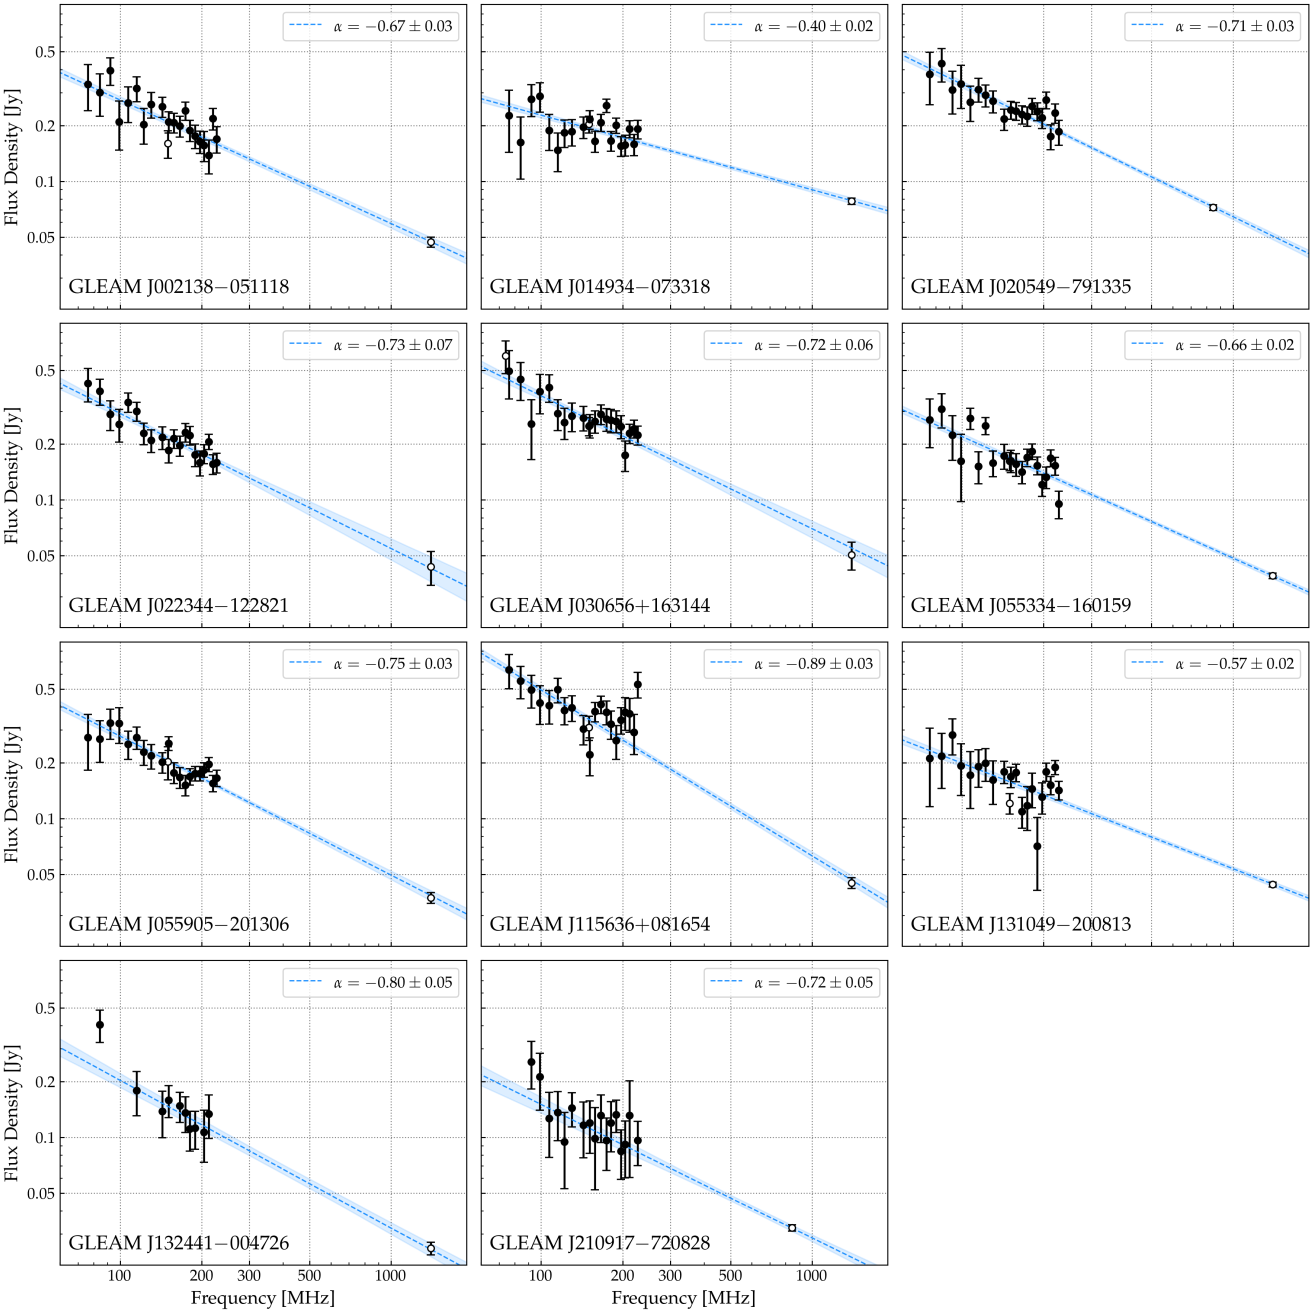


**Figure A1.** SED plots for the 12 GLEAM sources with large fractional uncertainty in `int_flux_fit_200`. Black markers denote GLEAM measurements, white markers denote measurements from the literature, using catalogues from TGSS-ADR1, SUMSS and the NVSS, where available. Dashed blue line denotes the best-fit power-law spectral index; shaded region denotes the $1\sigma$ uncertainty region mapped by `EMCEE`. All subplots are shown on matching $x$- and $y$-ranges.

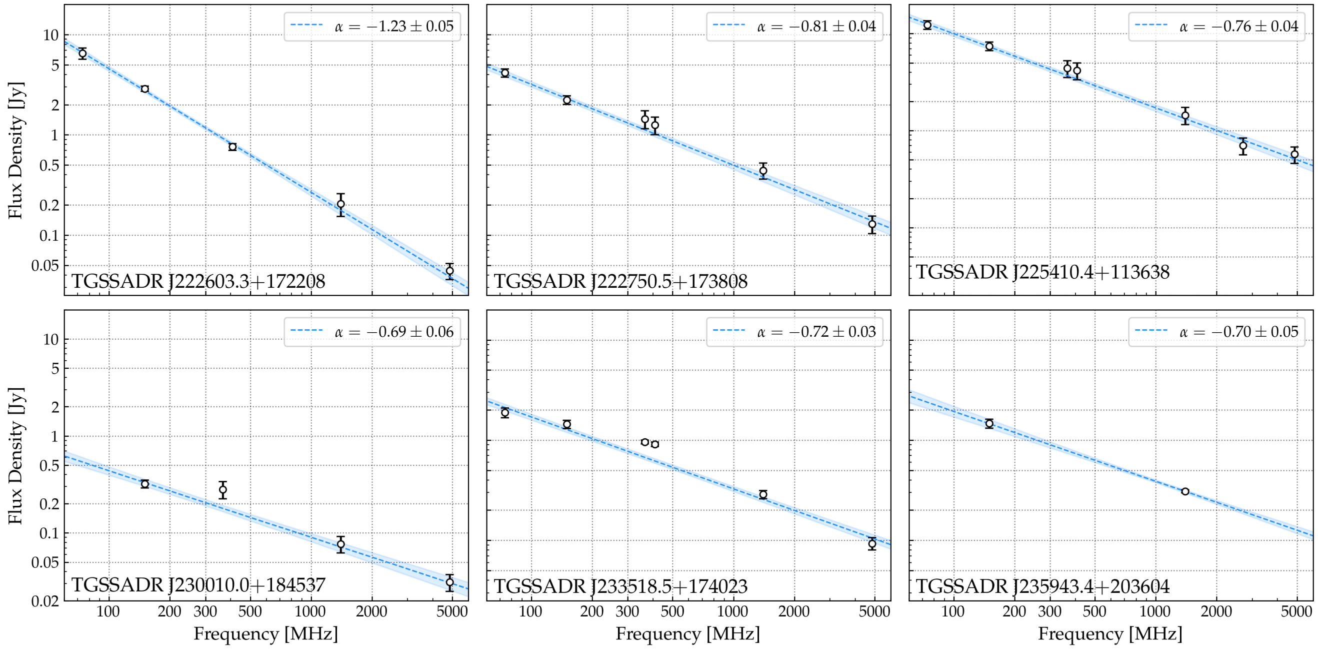


**Figure A2.** SED plots for sources detected using the TGSS-ADR1 Catalogue as a positional prior. White markers denote flux density measurements from the literature, using catalogues from the VLSSr, TGSS-ADR1, TXS, MRC, NVSS and GB6 surveys. Dashed blue line denotes the best-fit power-law spectral index; shaded region denotes the $1\sigma$ uncertainty region mapped by `EMCEE`. All subplots are shown on matching $x$- and $y$-ranges.

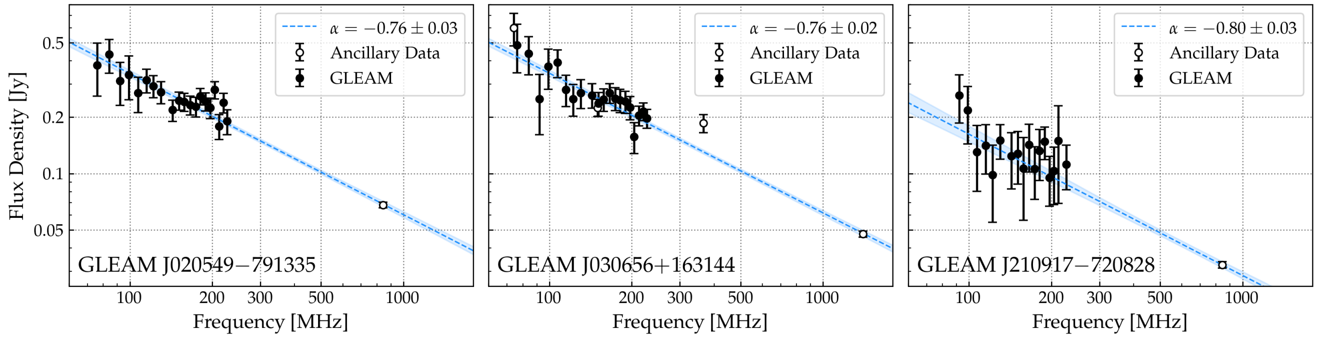


**Figure A3.** SED plots for three of the four pulsar candidates in our catalogue. The SED for our fourth pulsar candidate, TGSSADR J230010.0+184537, is already shown in Figure A2. Filled points denote flux density measurements from GLEAM, empty points denote ancillary measurements from various radio surveys. Dashed blue line denotes the best-fit power-law spectral index; shaded region denotes the $1\sigma$ uncertainty region mapped by `EMCEE`. All subplots are shown on matching $x$- and $y$-ranges.
