# Supplementary material for: The POlarised GLEAM Survey (POGS) II: Results from an All-Sky Rotation Measure Synthesis Survey at Long Wavelengths
Source: arXiv:2005.09266 ancillary file (2020-11-12)
Supplement: Supplementary file 2 [file Appendix-B.pdf]

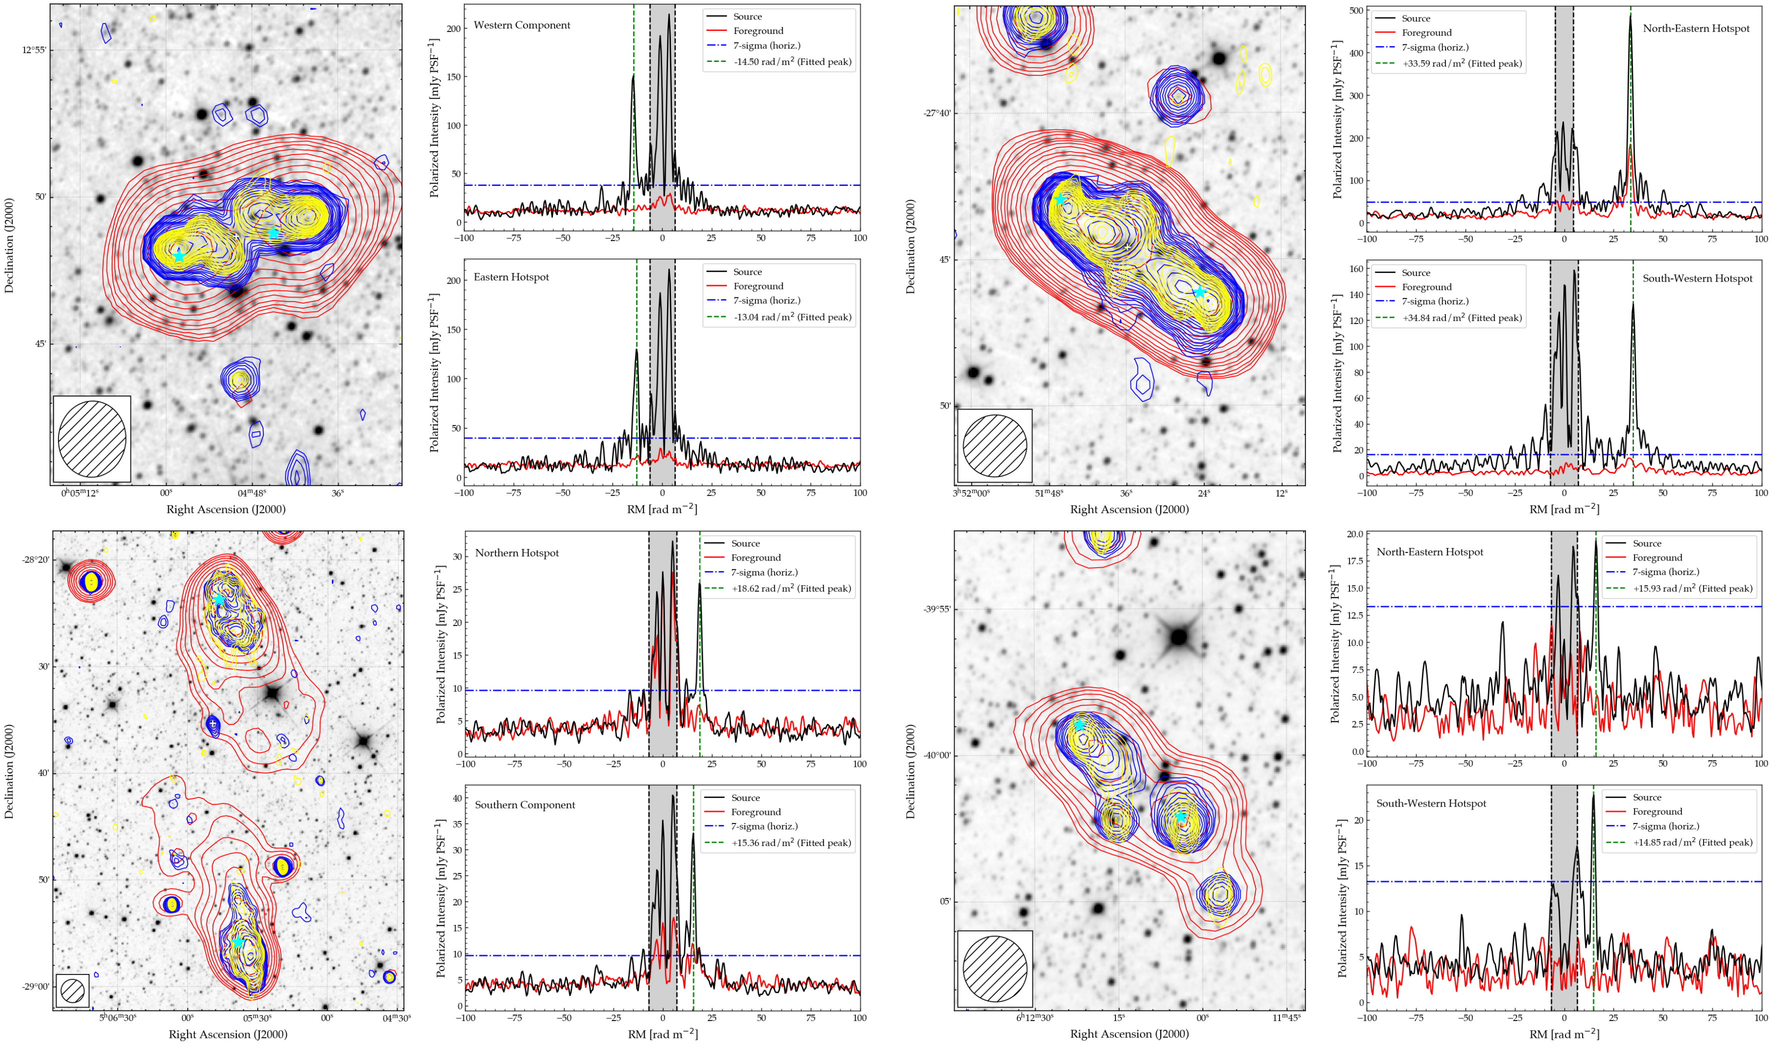


**Figure B1.** POGS ExGal 'Polarised doubles'. Panels show the following sources: POGSII-EG-005 & POGSII-EG-006 (G4Jy 7; *top left*), POGSII-EG-152 & POGSII-EG-153 (PMN J0351−2744/G4Jy 386; *top right*), POGSII-EG-174 & POGSII-EG-175 (ESO 422−G028/MSH 05-22/G4Jy 517; *bottom left*) and POGSII-EG-210 & POGSII-EG-211 (*bottom right*). Red, blue and yellow contours denote Stokes $I$ surface brightness from GLEAM (200 MHz), the NVSS and TGSS-ADR1 respectively, starting at $3\sigma$ and scaling by a factor $\sqrt{2}$. Where a host galaxy could be found, it is identified by a white '+'. Note that a host could not confidently be identified for POGSII-EG-210 & POGSII-EG-211. Right panels in each subplot show the source RM spectrum along the LOS through the cyan star (black) plus the foreground RM spectrum (red) as well as the instrumental leakage avoidance zone (shaded gray region). Green dashed line denotes the fitted RM; blue dot-dashed line denotes the $7\sigma$ level.

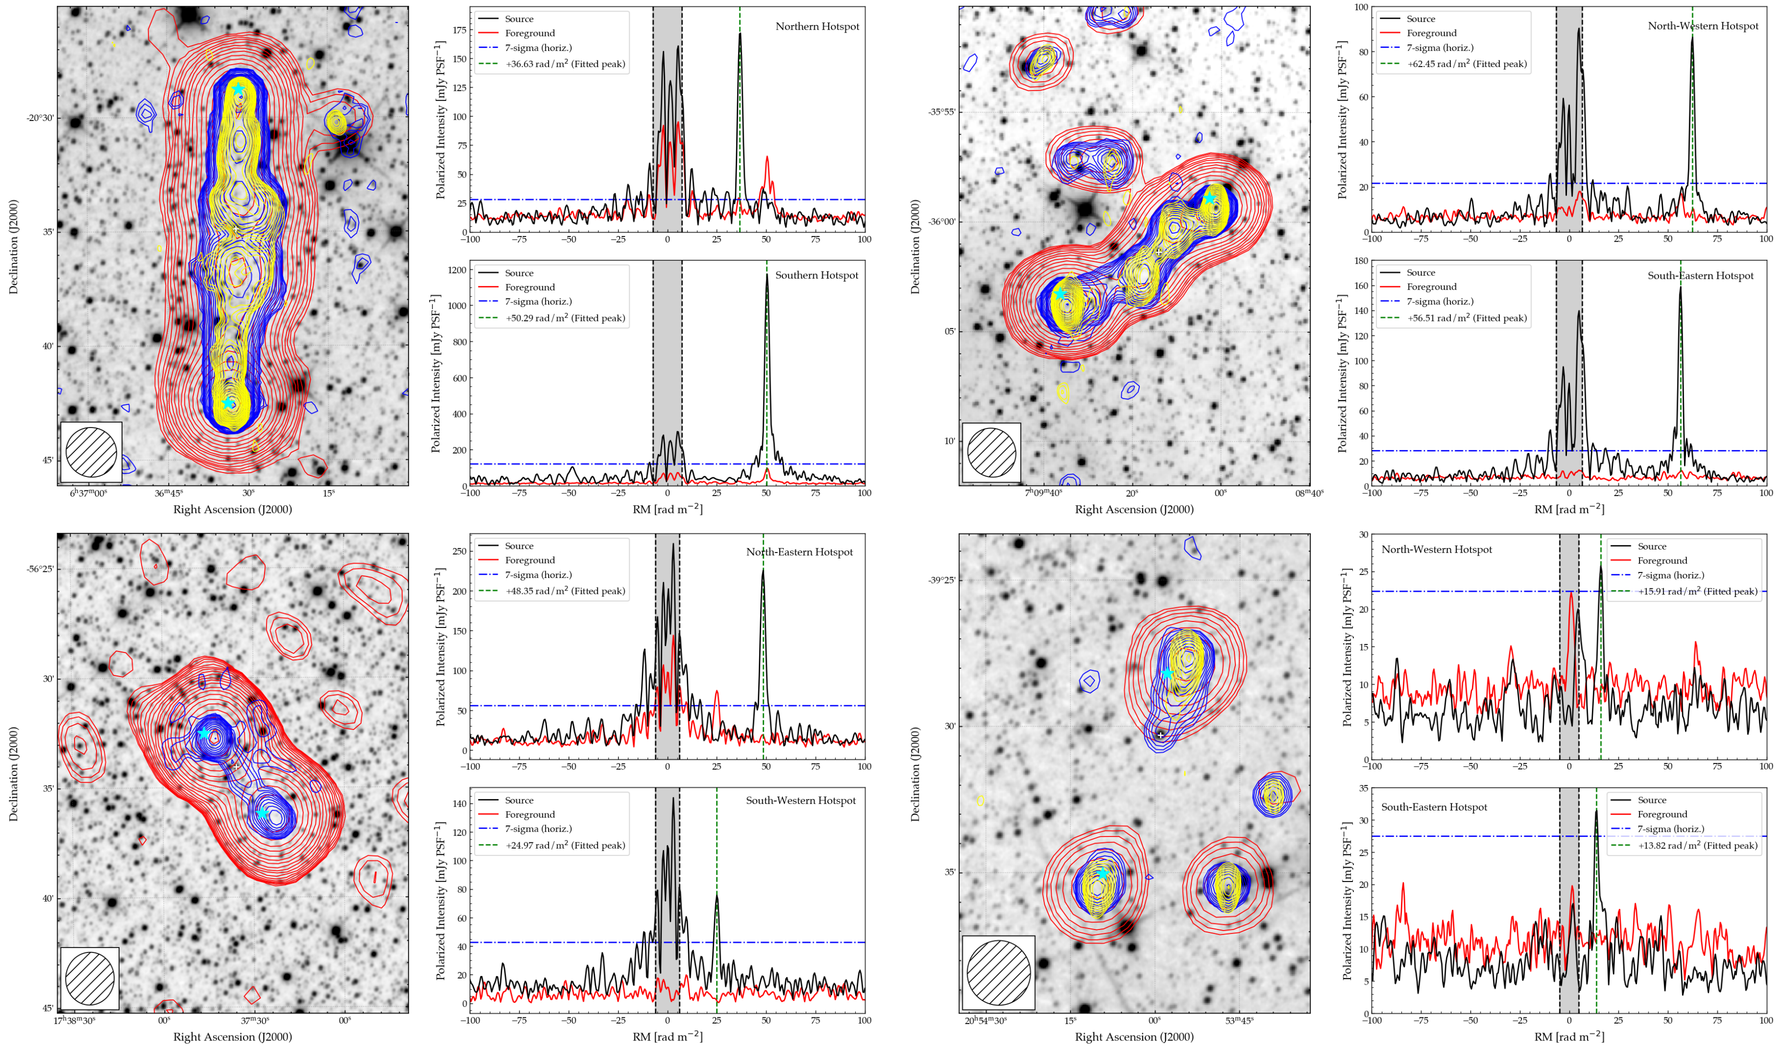


**Figure B1.** (*continued*). Panels show the following sources: POGSII-EG-221 & POGSII-EG-222 (PKS J0636−2036/G4Jy 619; *top left*), POGSII-EG-235 & POGSII-EG-236 (PKS 0707−35/G4Jy 644; *top right*), POGSII-EG-365 & POGSII-EG-366 (PKS 1733−56/G4Jy 1423; *bottom left*) and POGSII-EG-400 & POGSII-EG-401 (*bottom right*). Blue contours in the bottom left panel show SUMSS surface brightness starting at $20\sigma$ and scaling by a factor $\sqrt{2}$, due to the presence of strong artefacts associated with bright sources in SUMSS.
