# Supplementary material for: The POlarised GLEAM Survey (POGS) II: Results from an All-Sky Rotation Measure Synthesis Survey at Long Wavelengths
Source: arXiv:2005.09266 ancillary file (2020-11-12)
Supplement: Supplementary file 3 [file Appendix-D.pdf]

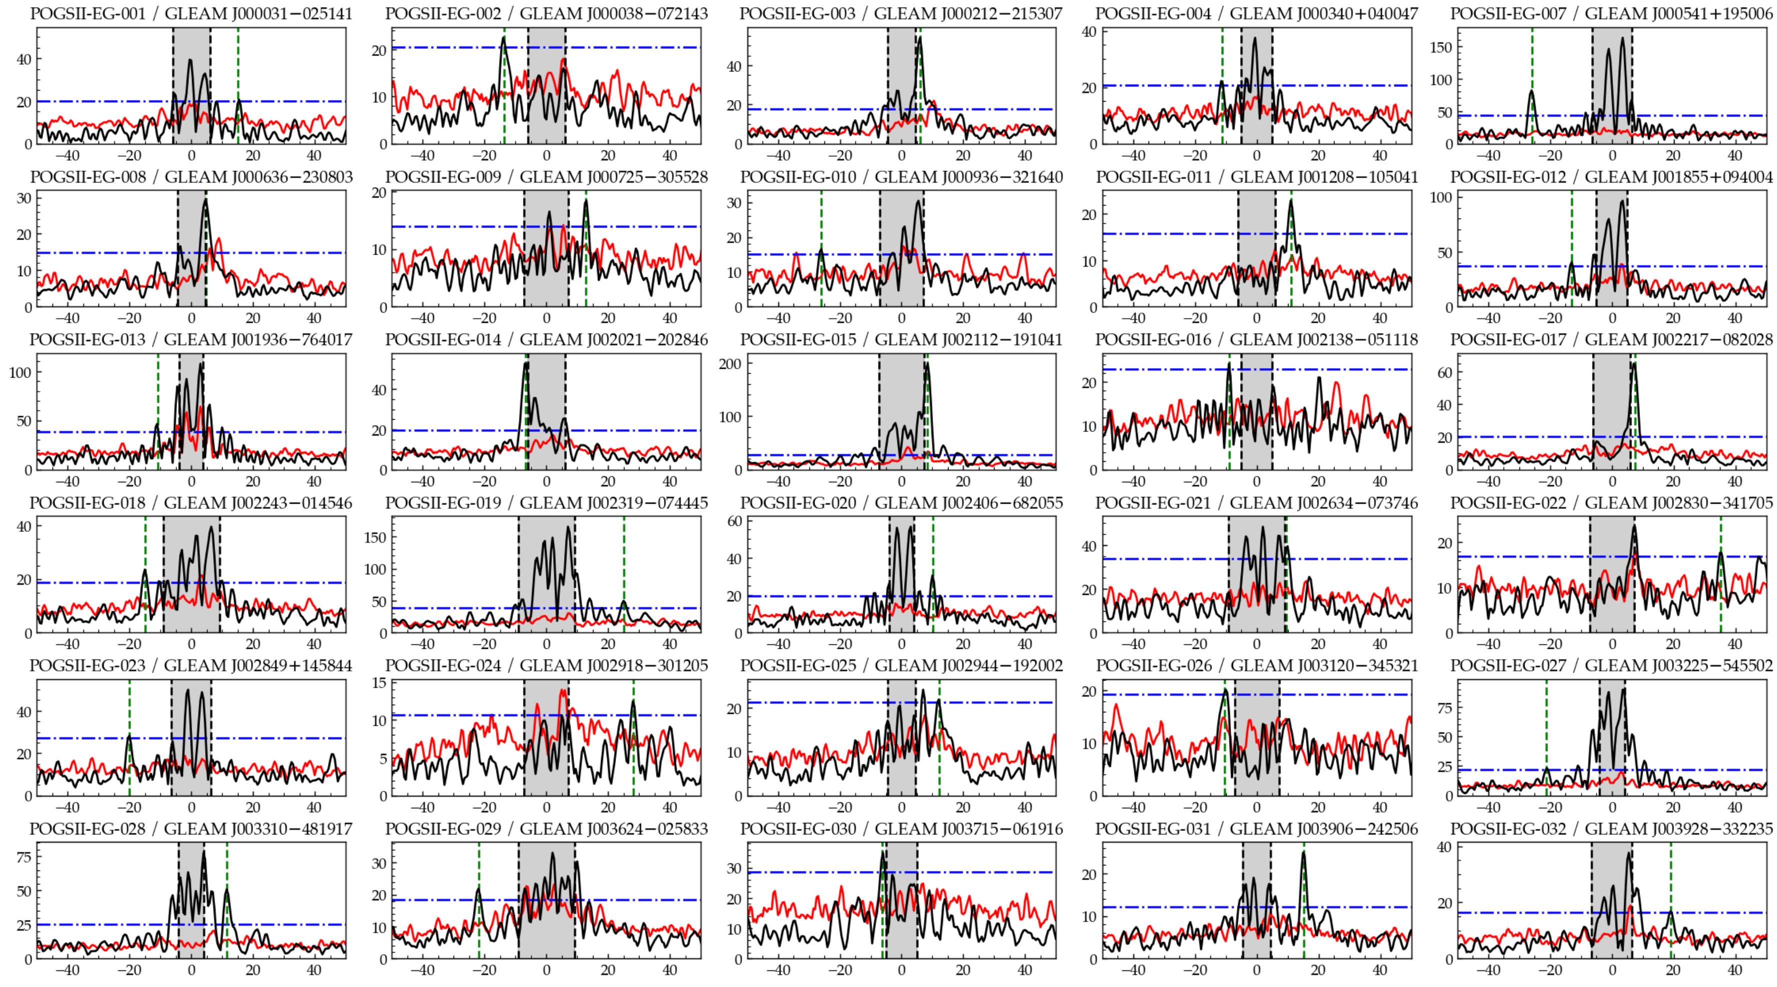


**Figure D1.** RM spectra for POGS ExGal sources. The x-axes show RM [rad m$^{-2}$], y-axes show linearly-polarised flux density [mJy beam$^{-1}$]. The source RM spectrum (off-source foreground RM) is shown in black (red). The instrumental leakage avoidance zone is shown in shaded gray; the green dashed line denotes the fitted RM, and the blue dot-dashed line denotes the 7$\sigma$ level.

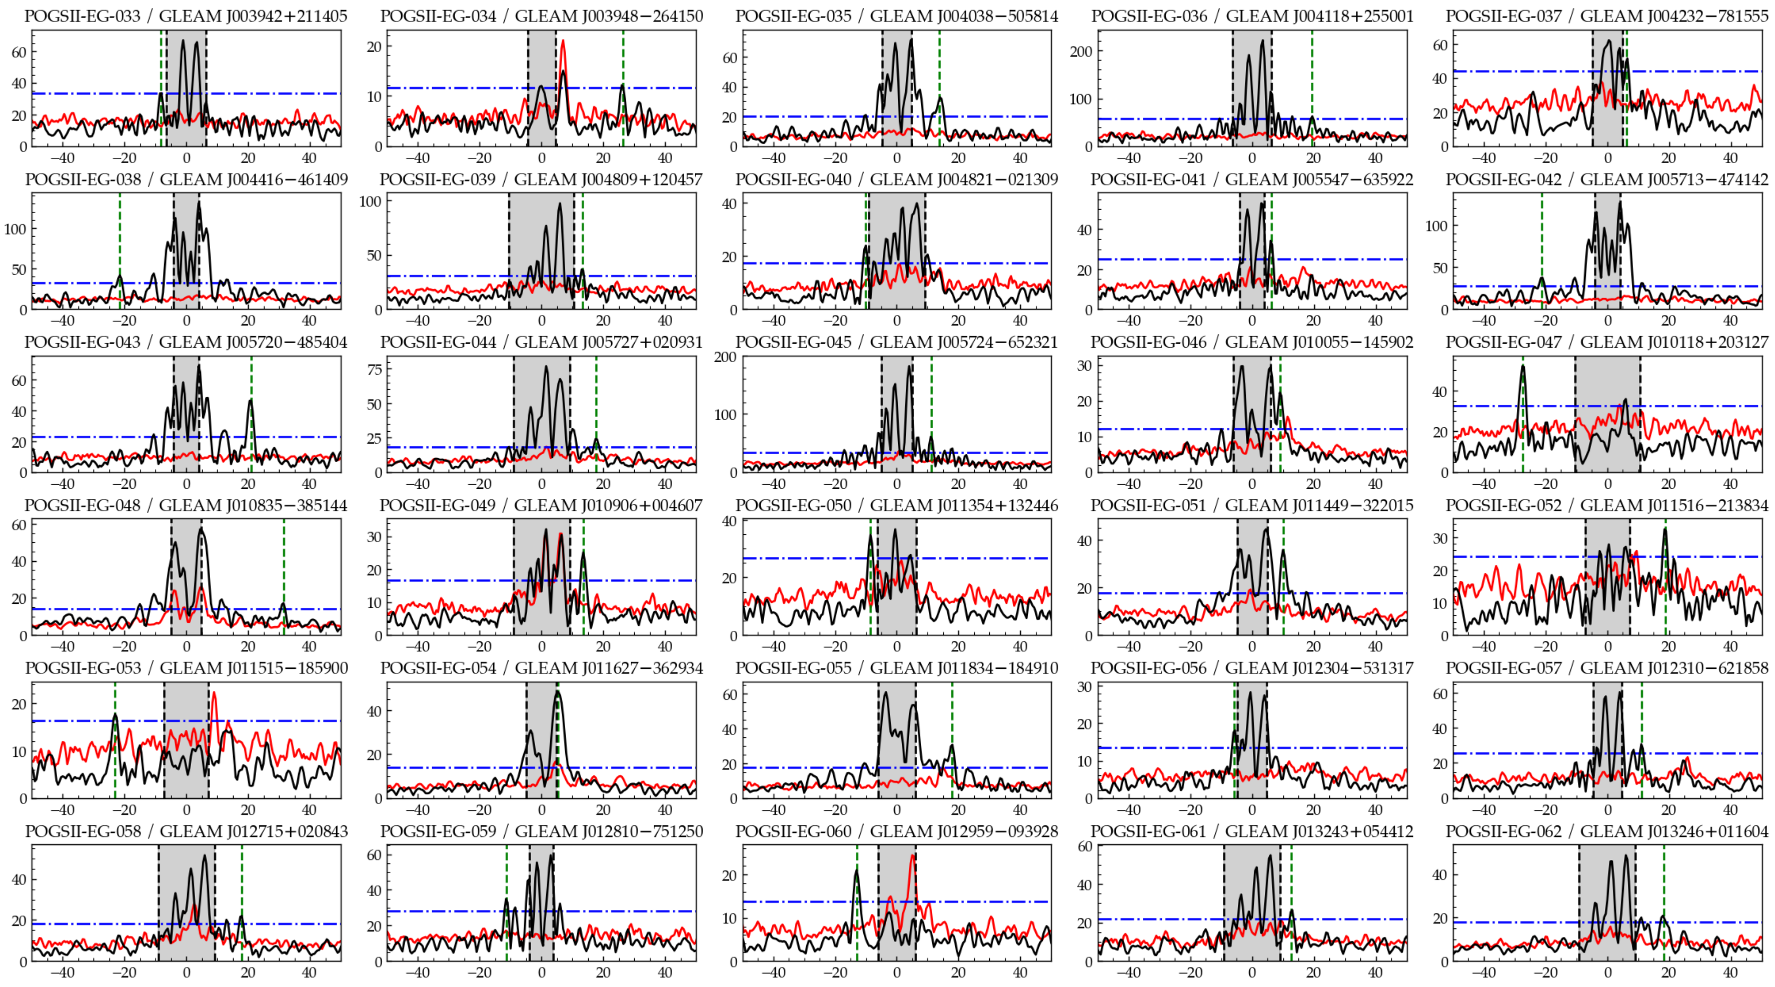


**Figure D1.** (*continued*)

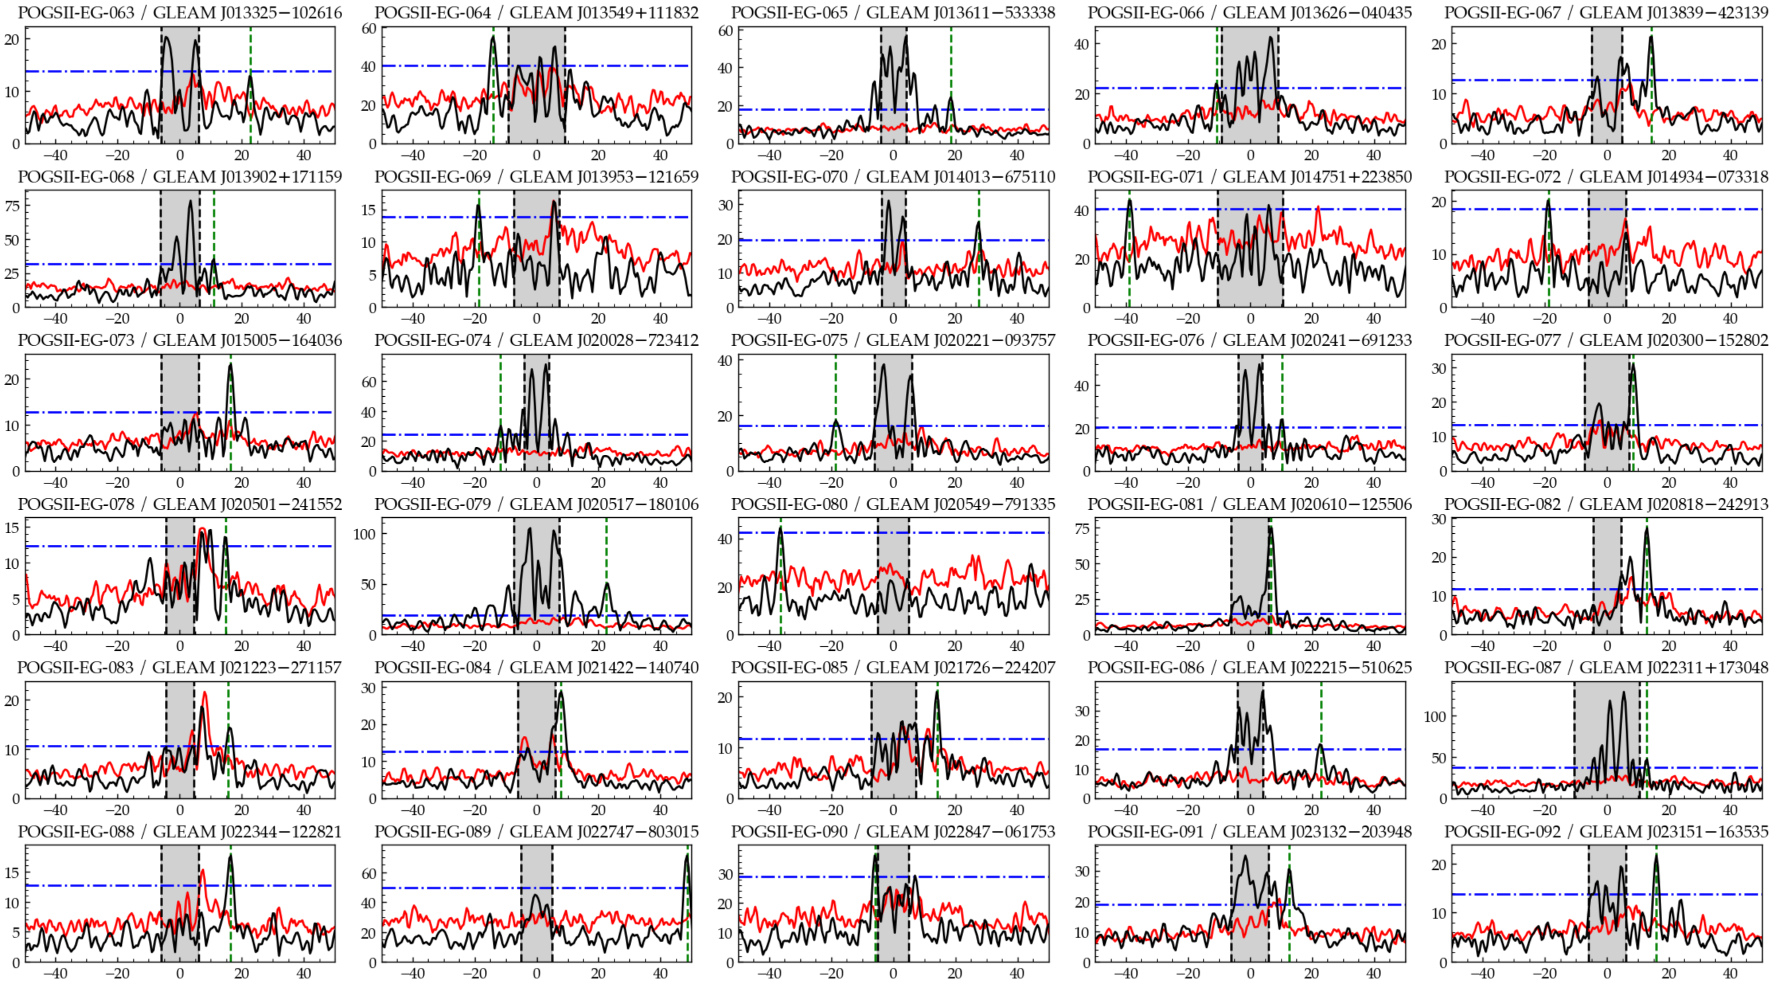


**Figure D1.** (*continued*)

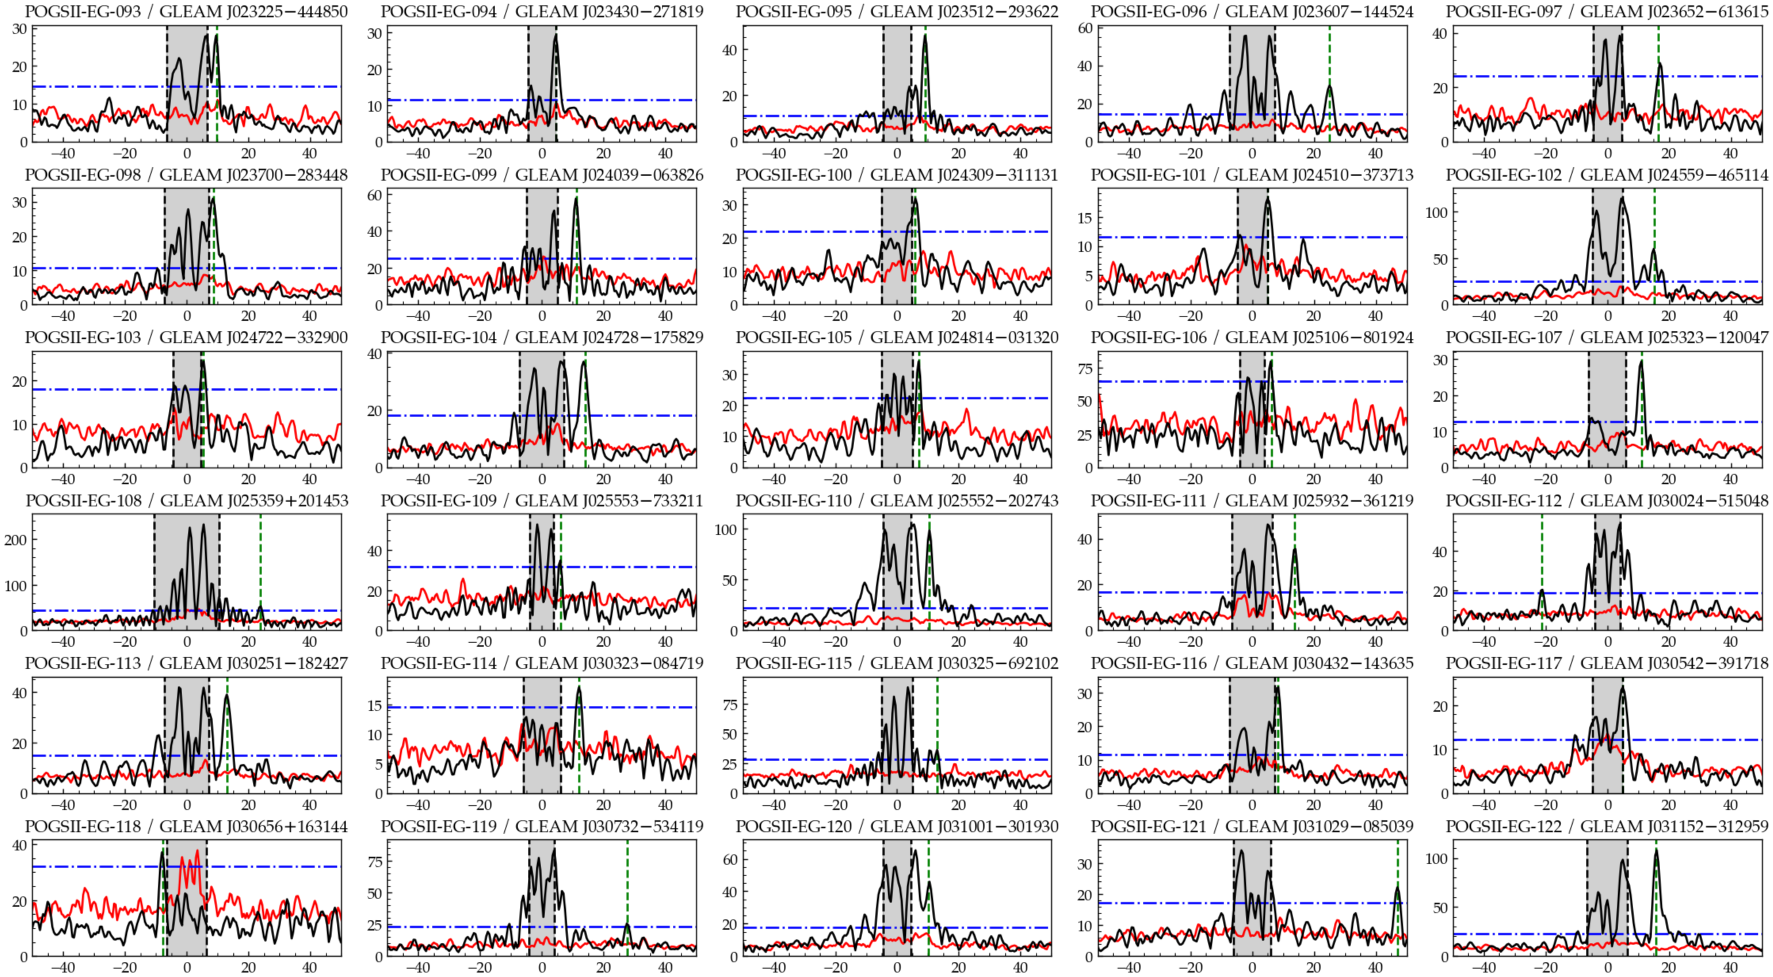


**Figure D1.** (*continued*)

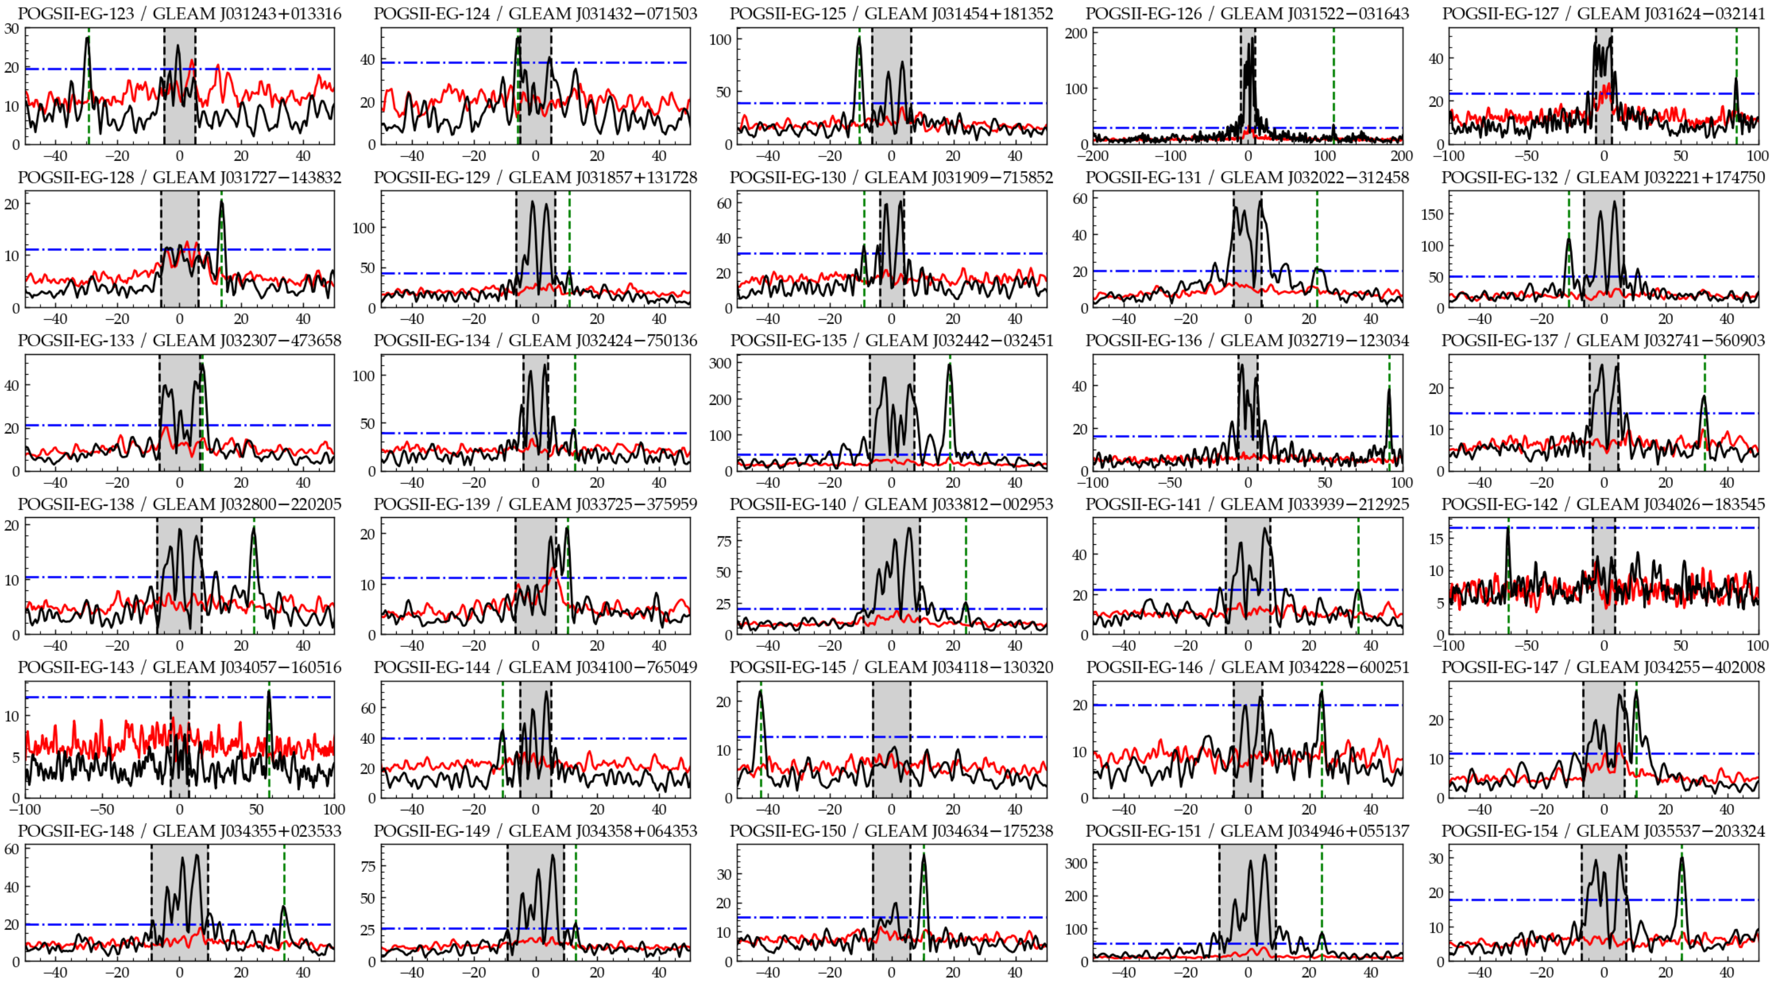


**Figure D1.** (*continued*)

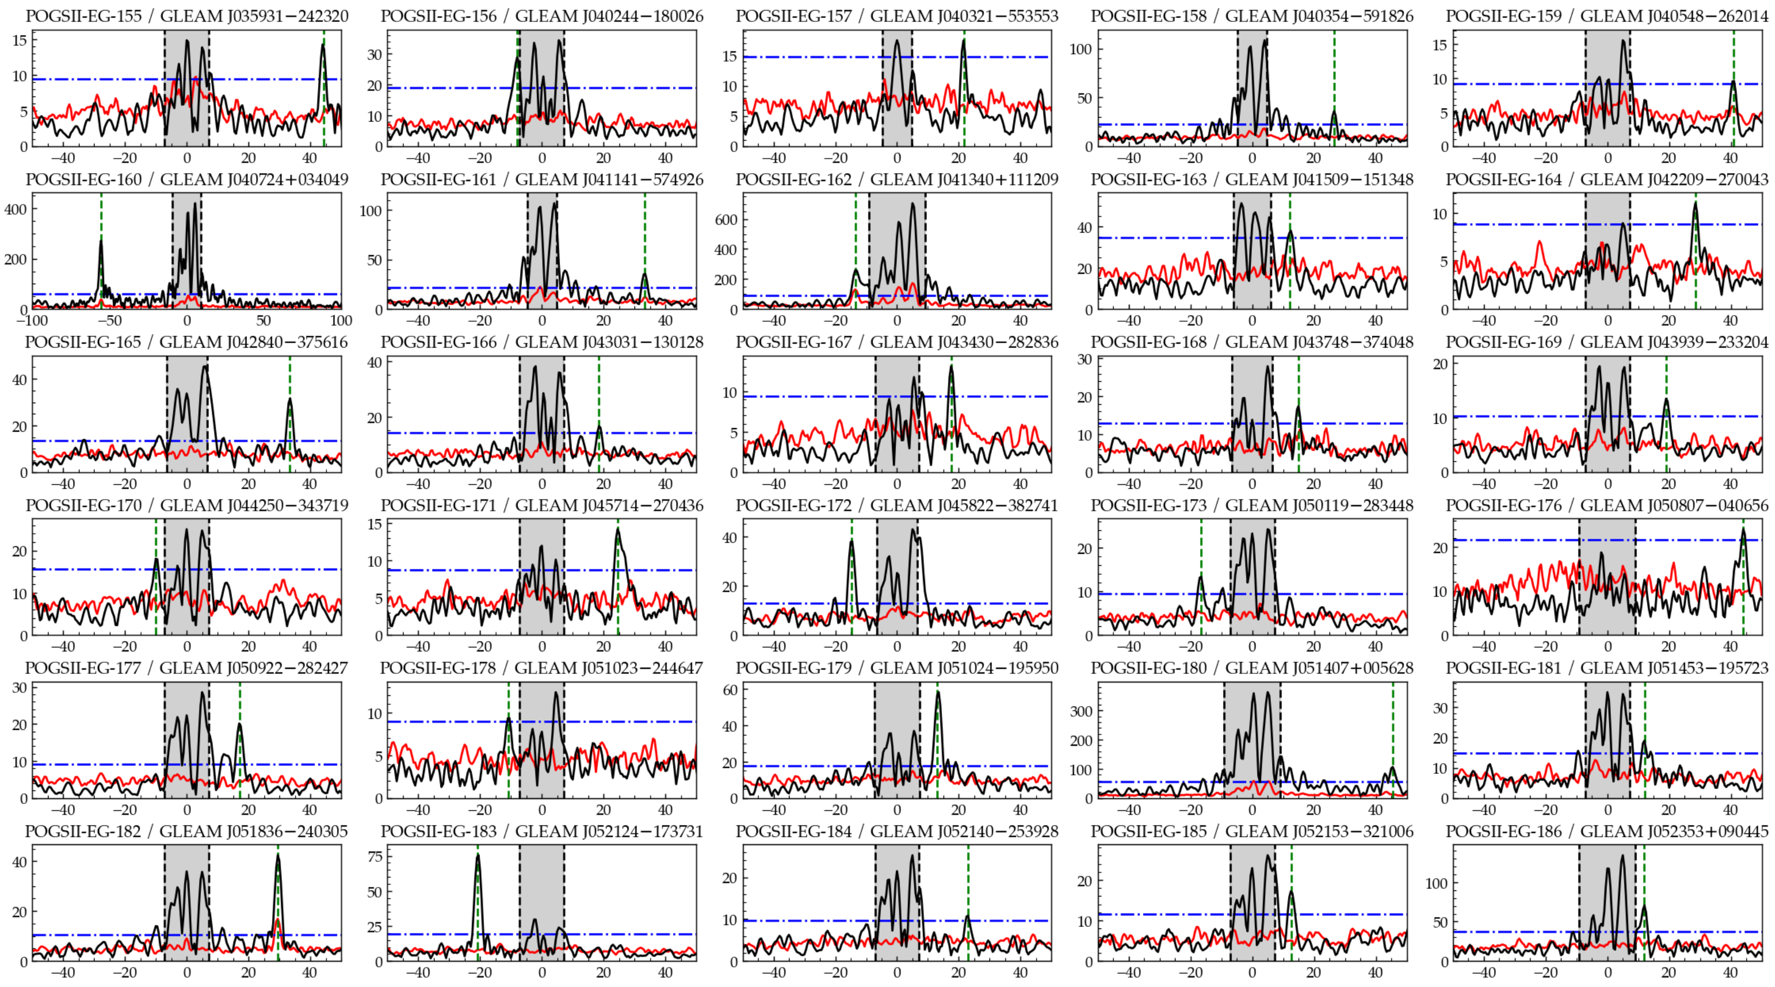


**Figure D1.** (*continued*)

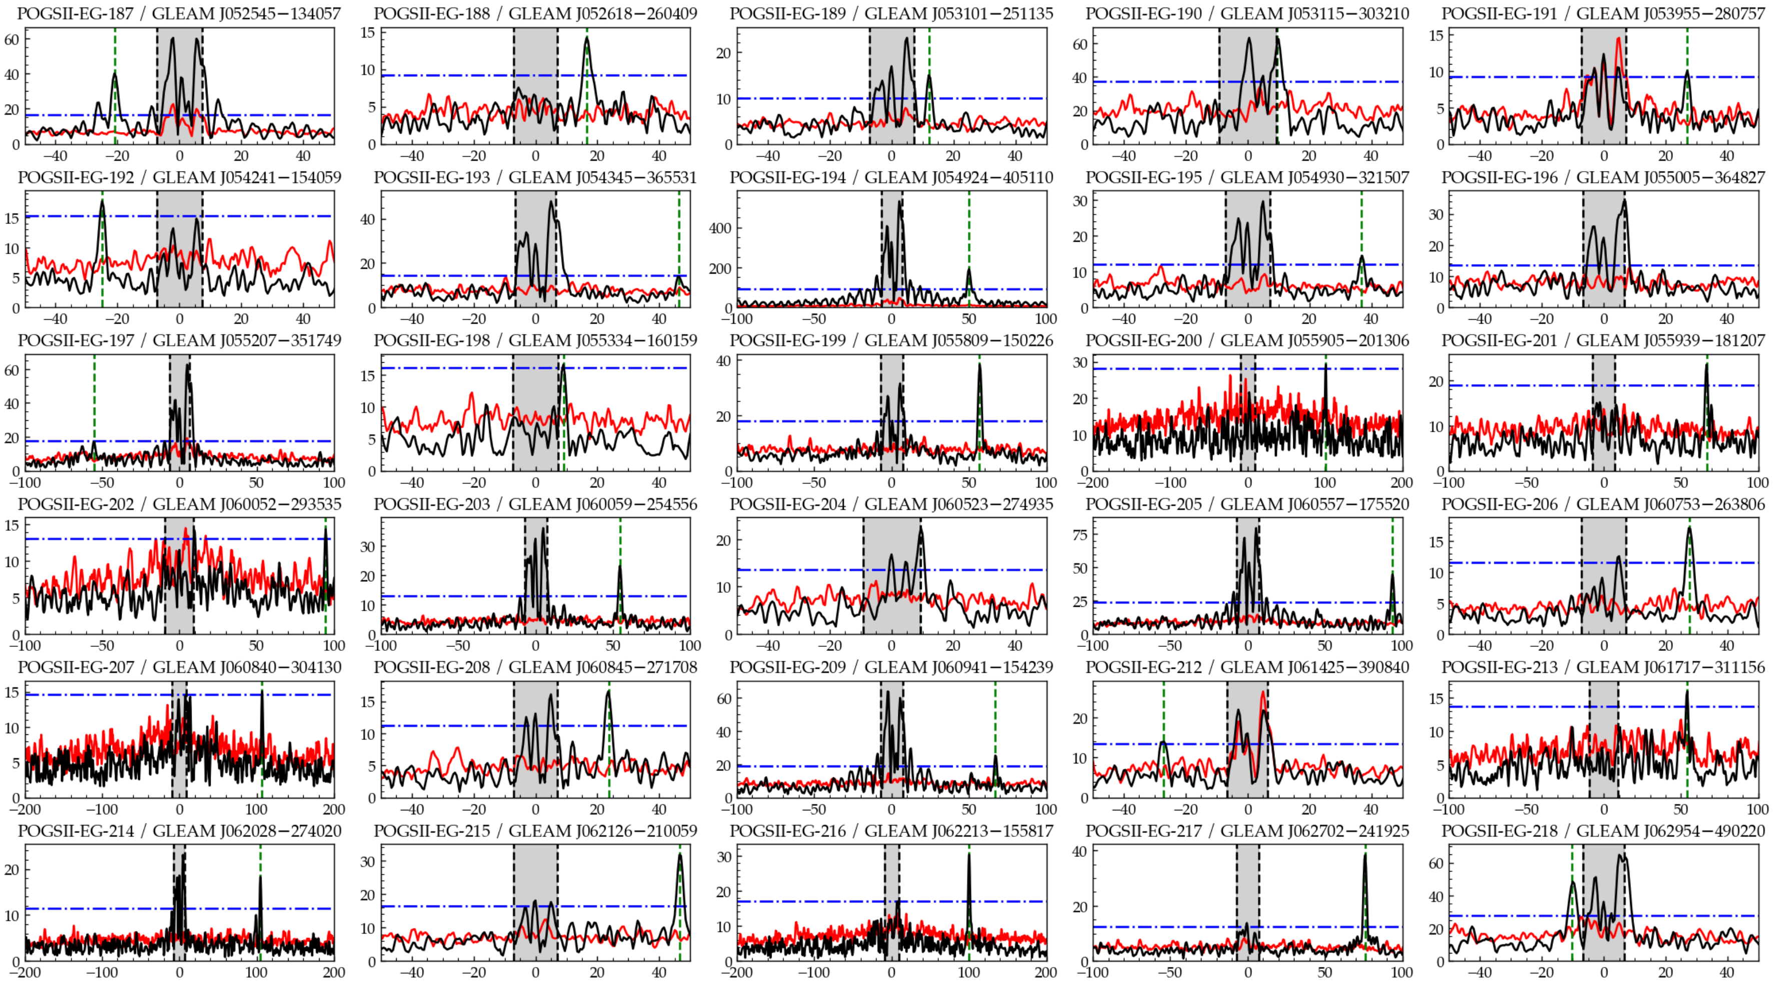


**Figure D1.** (*continued*)

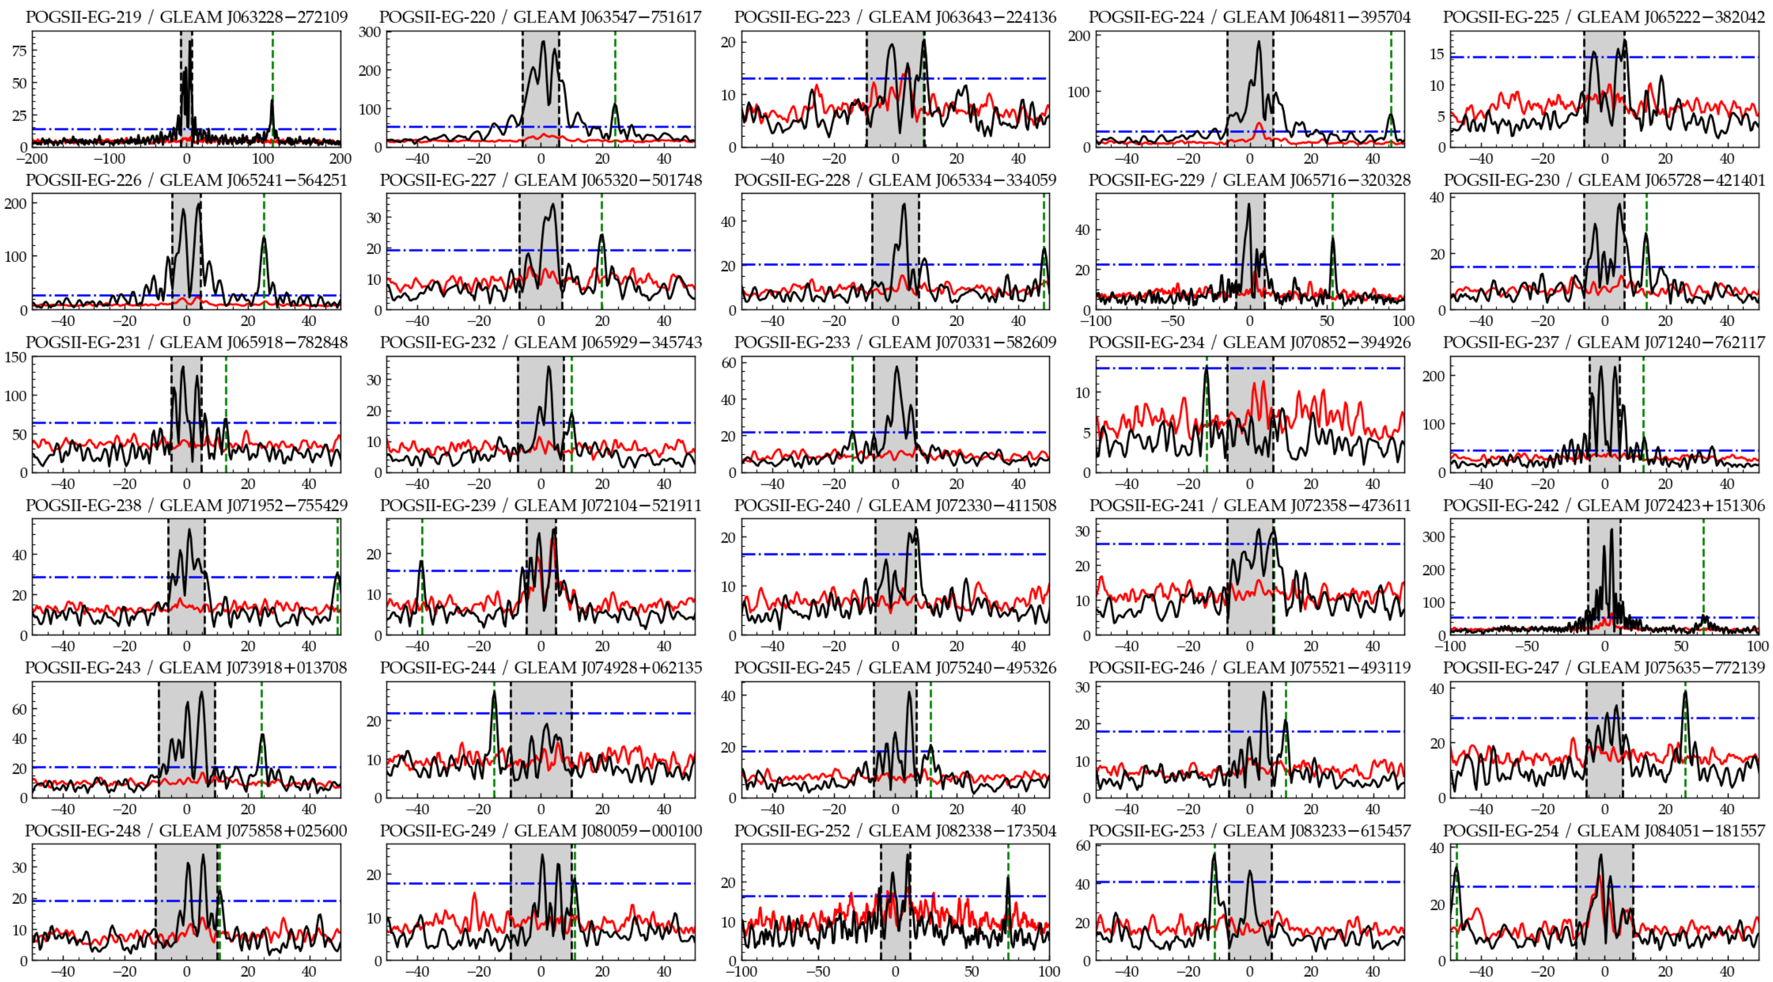


**Figure D1.** (*continued*)

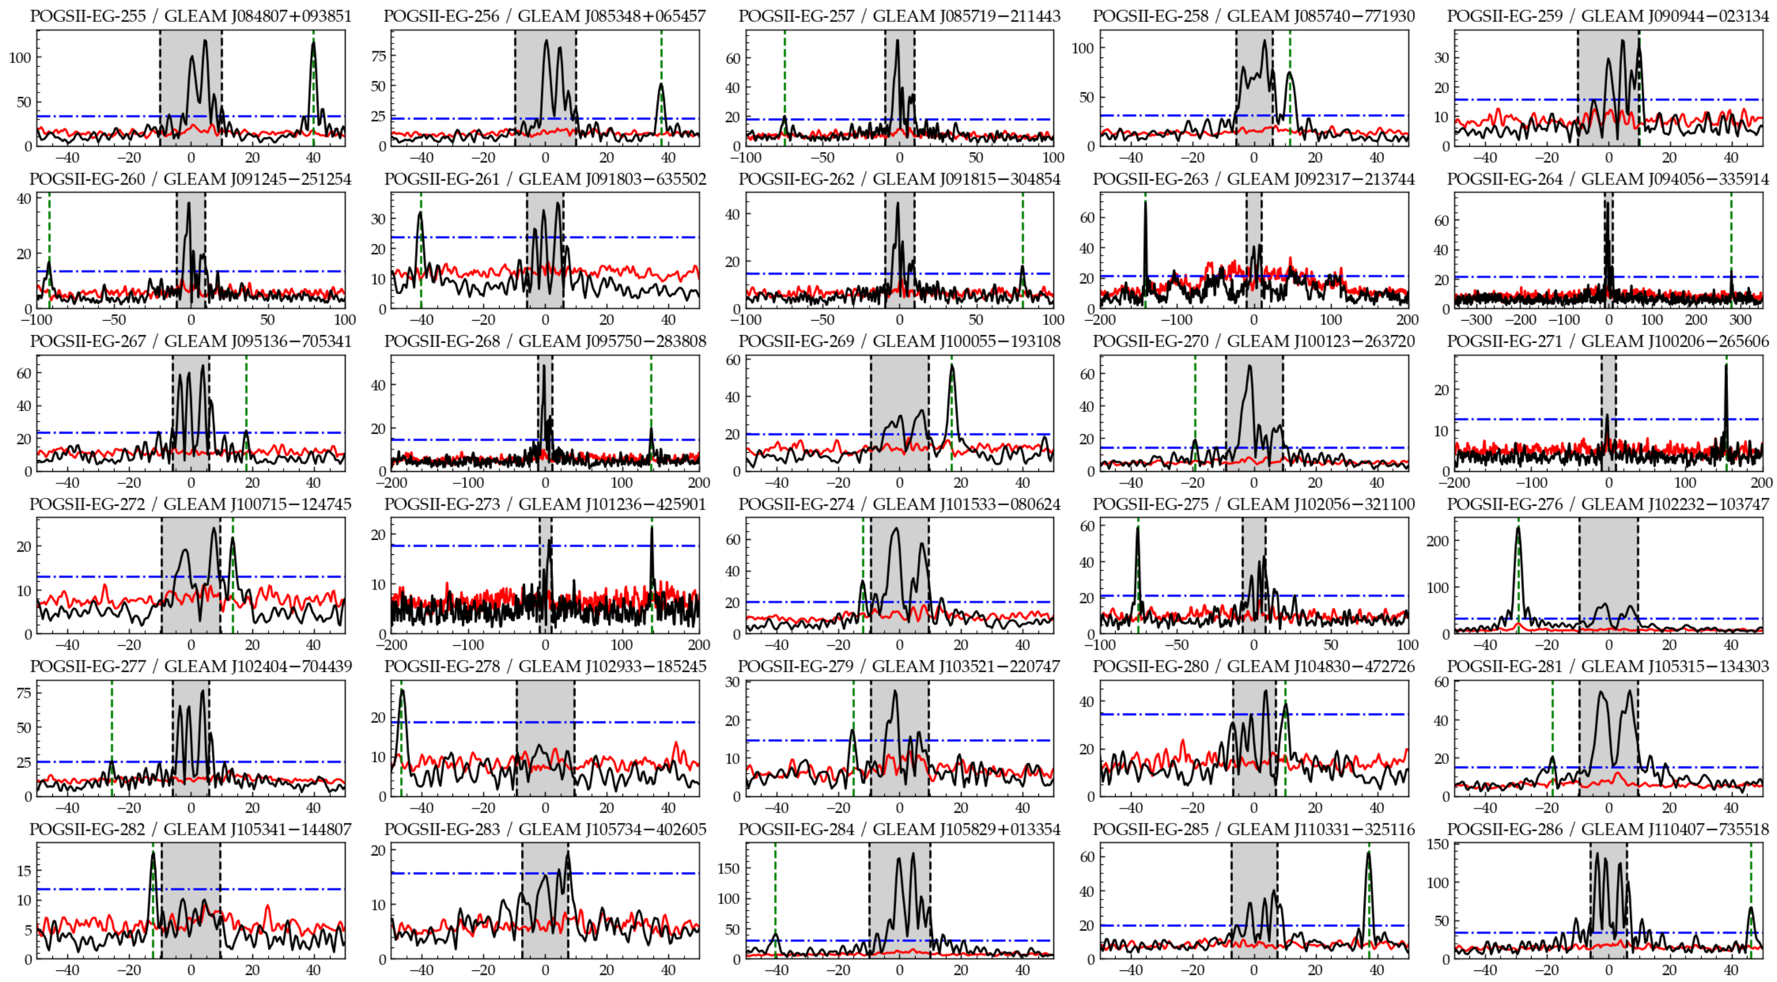


**Figure D1.** (*continued*)

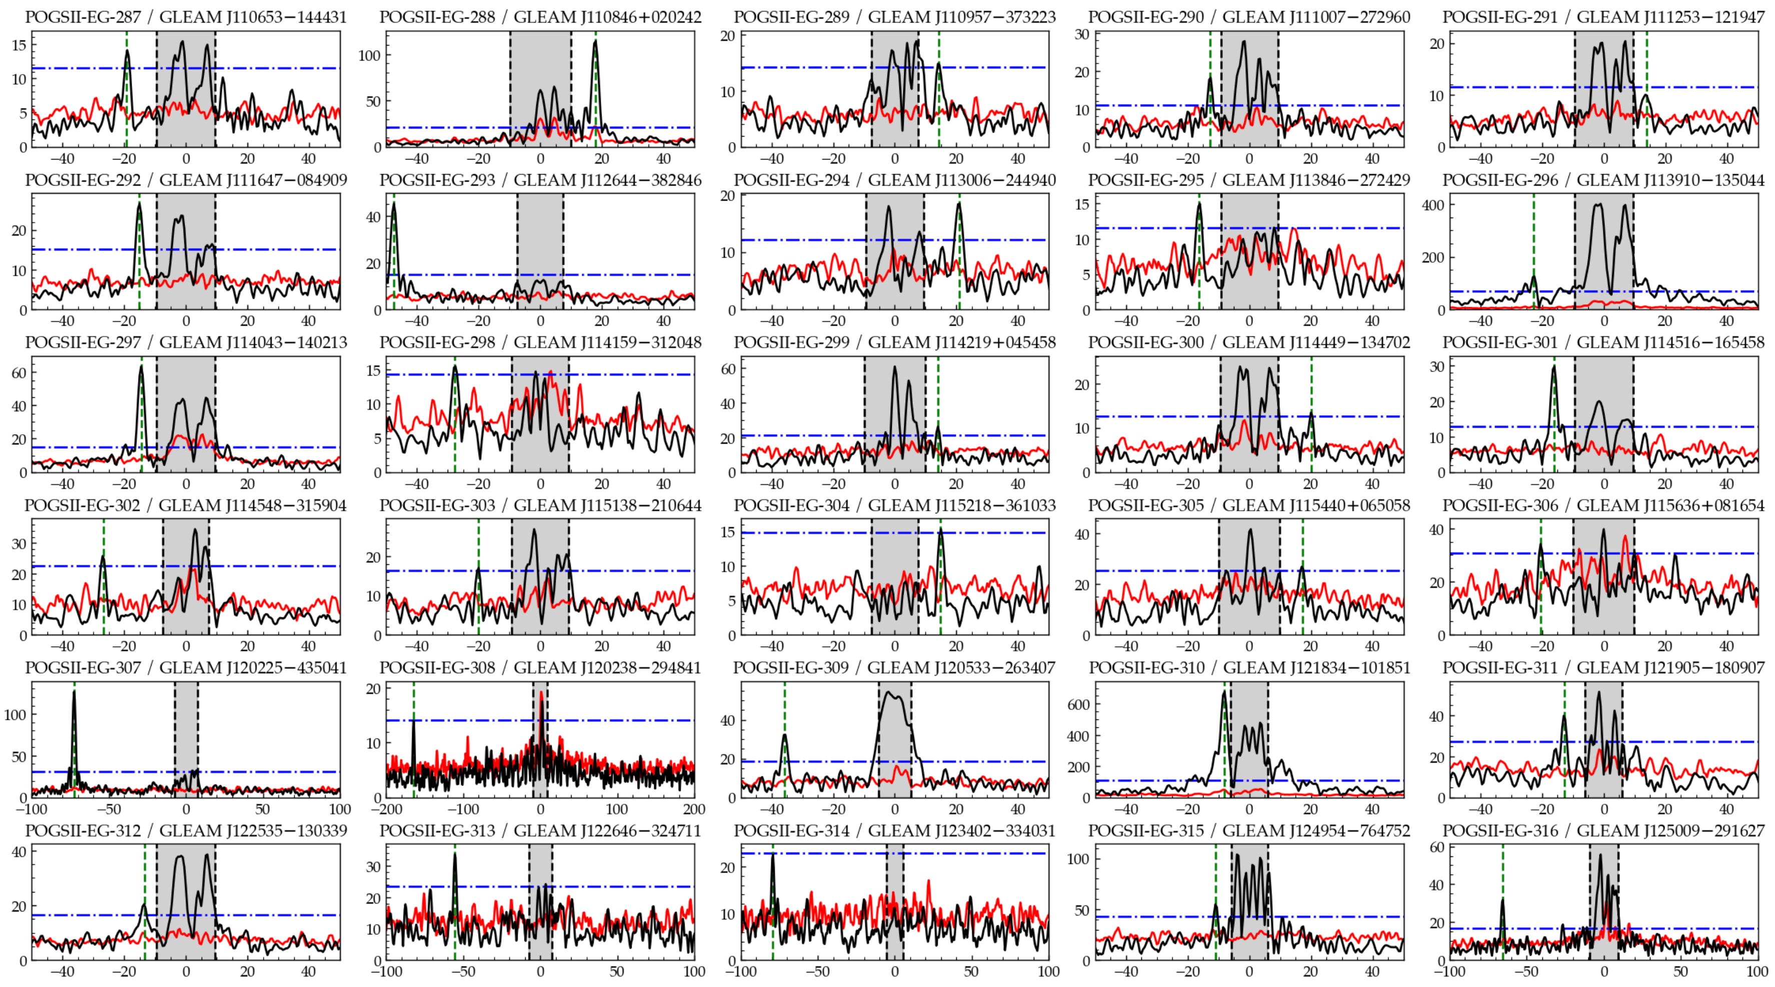


**Figure D1.** (*continued*)

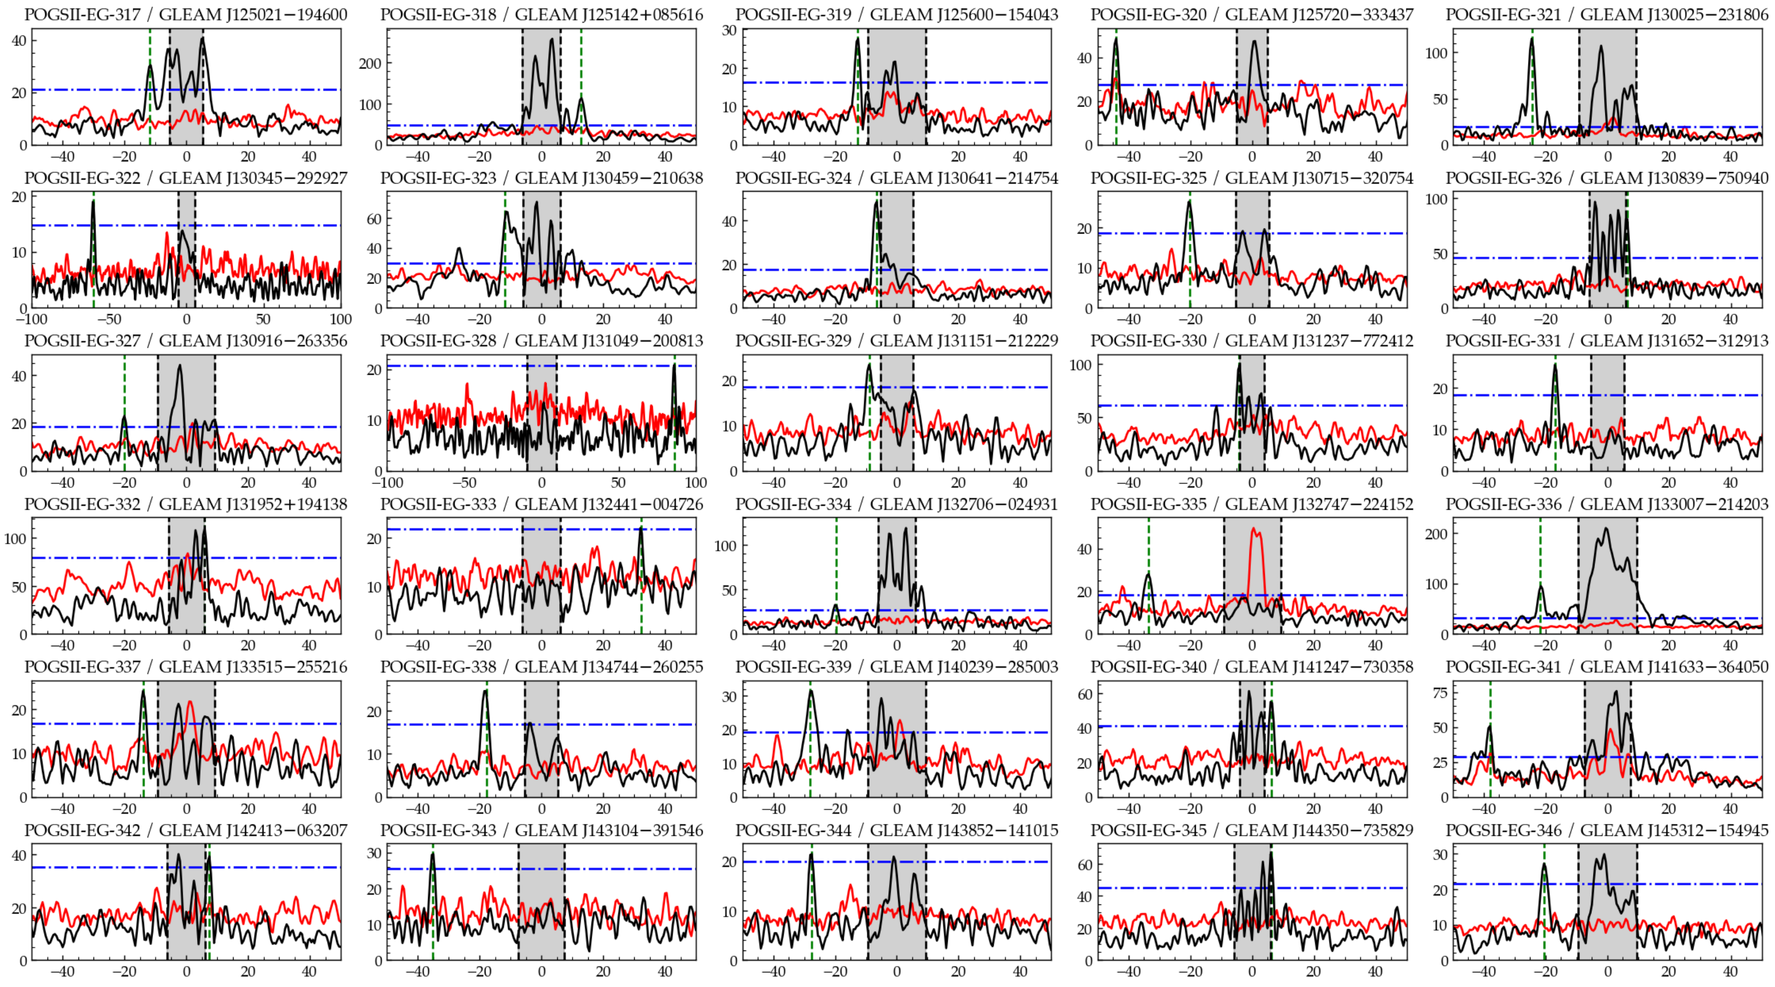


**Figure D1.** (*continued*)

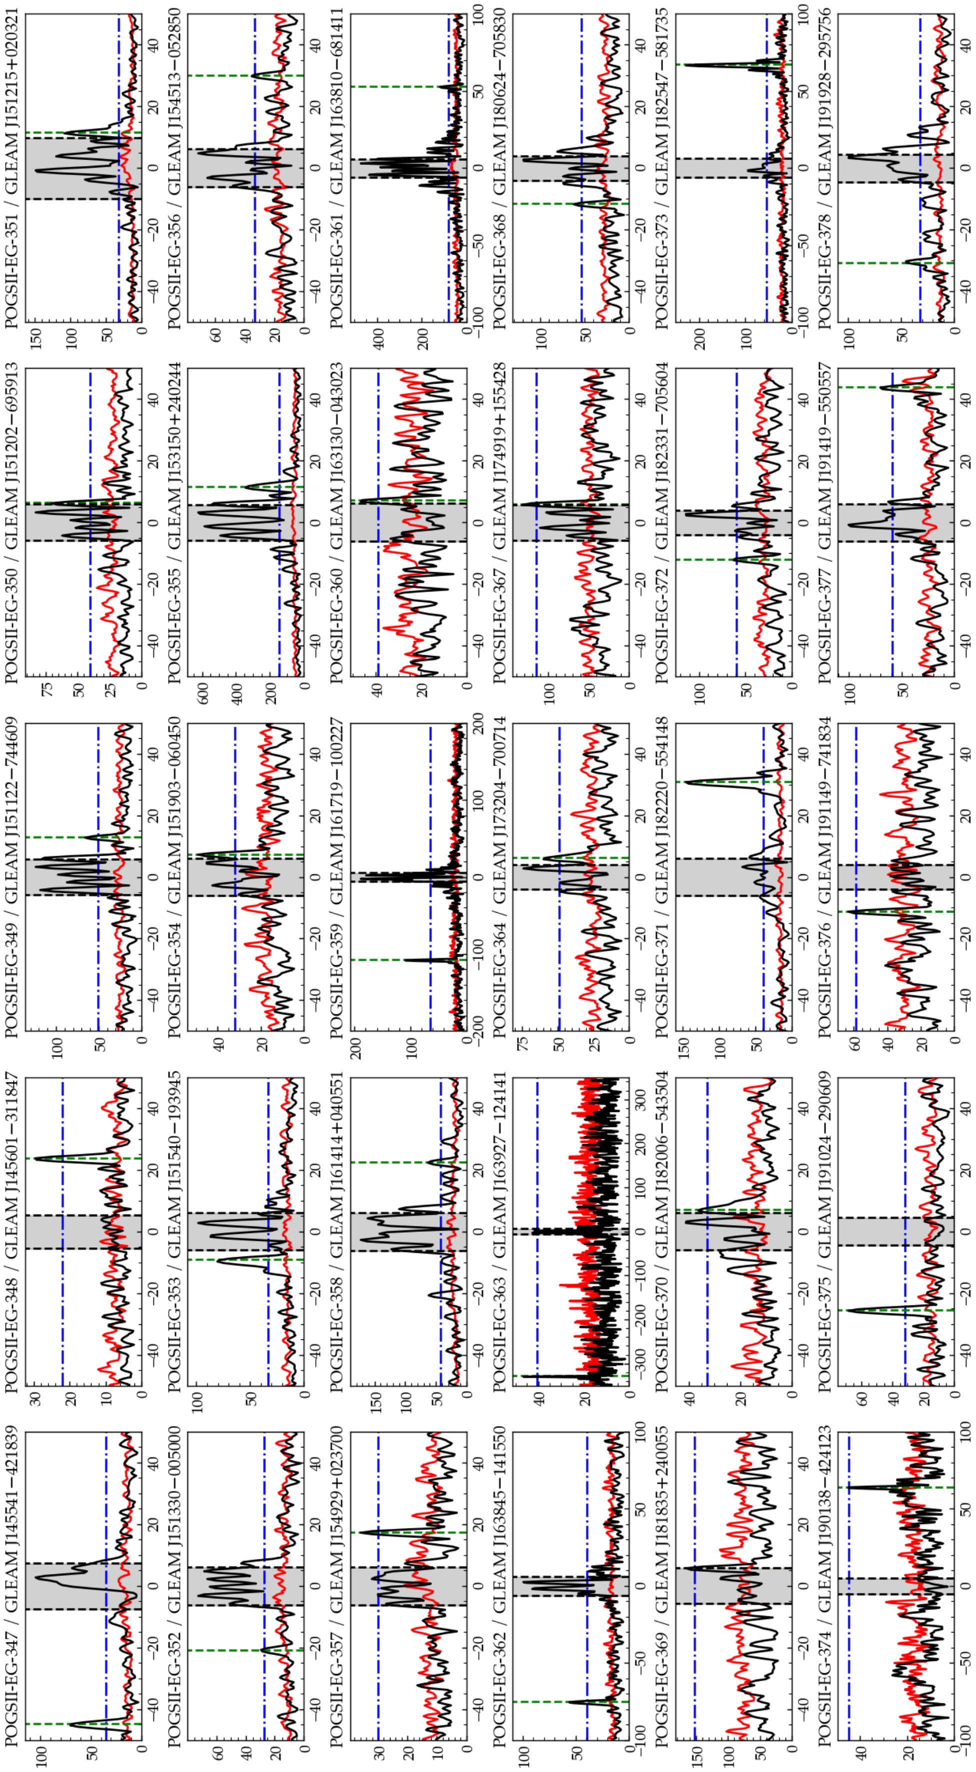


**Figure D1.** (*continued*)

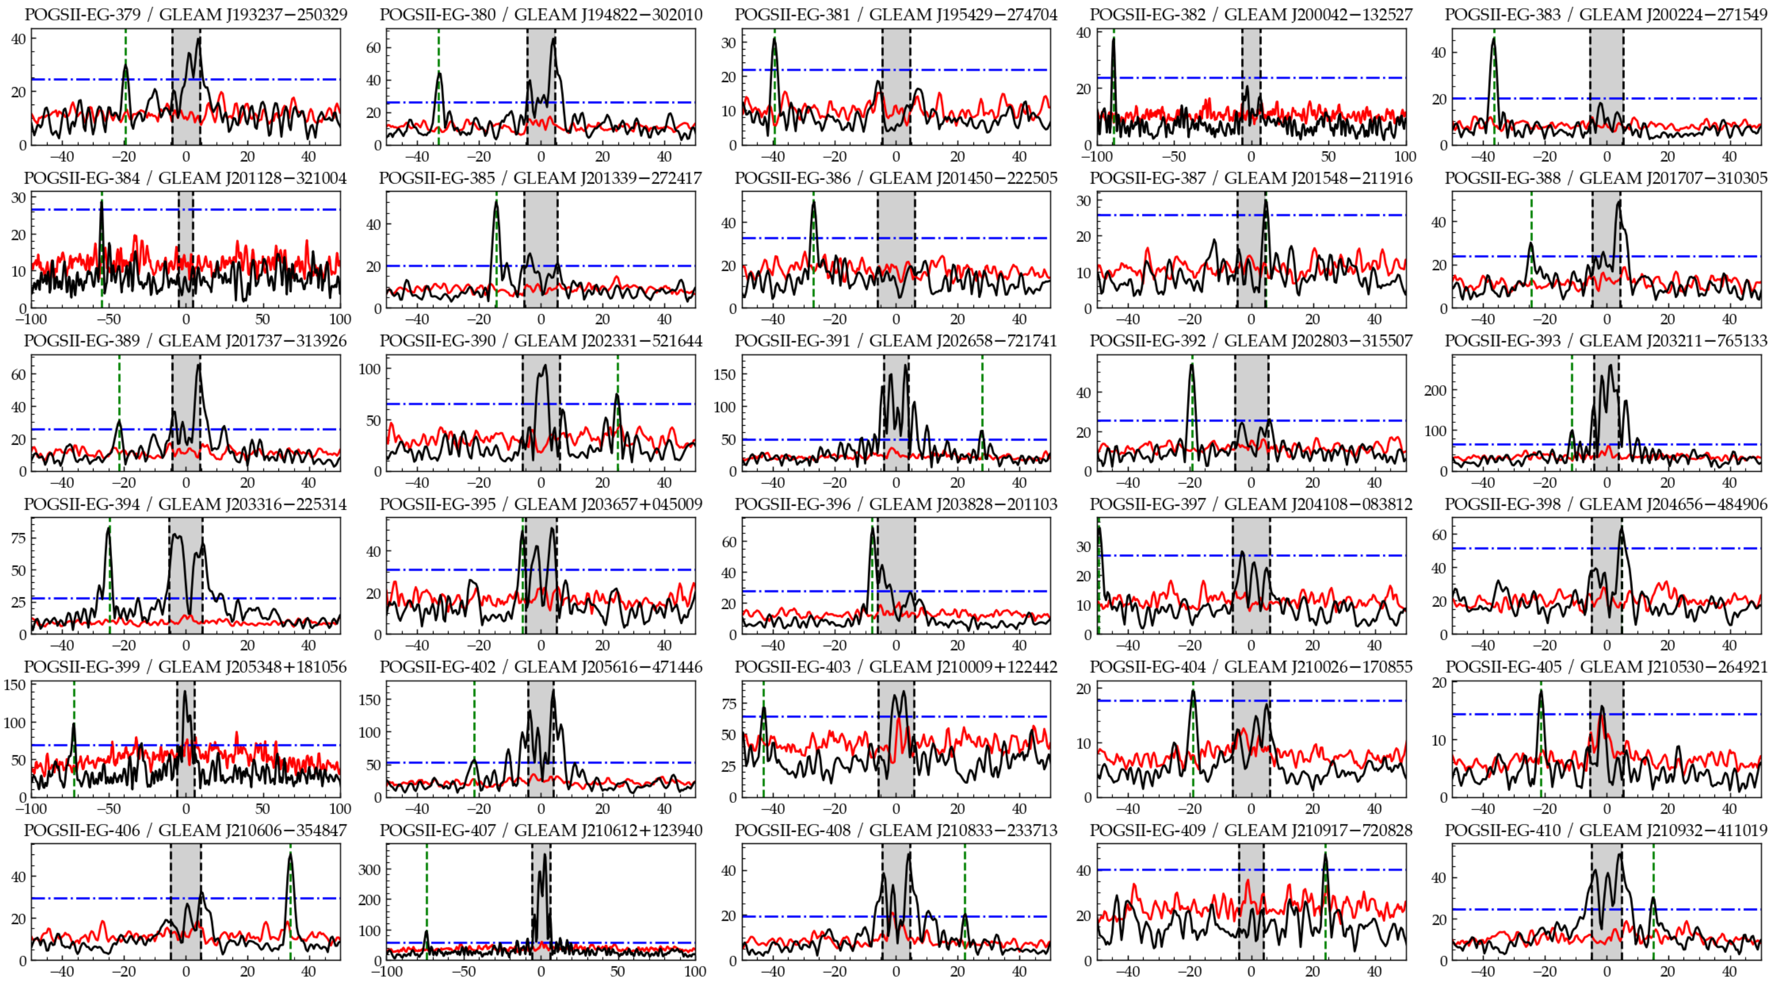


**Figure D1.** (*continued*)

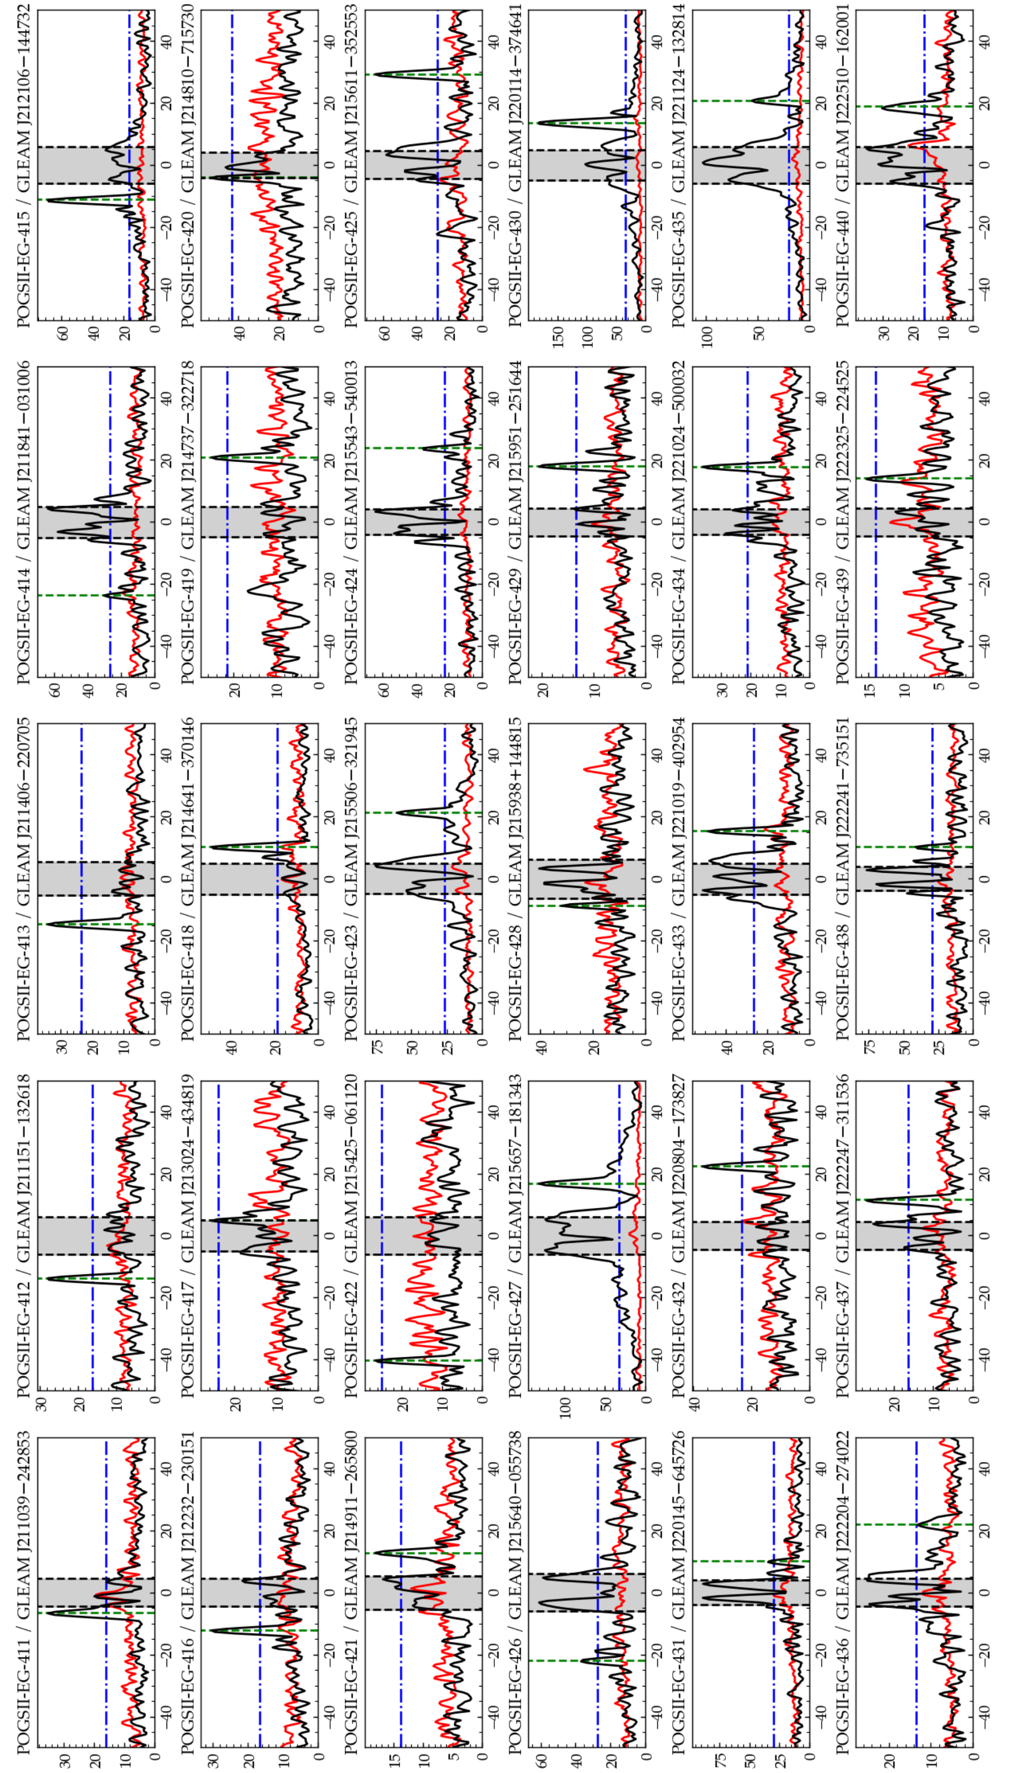


**Figure D1.** (*continued*)

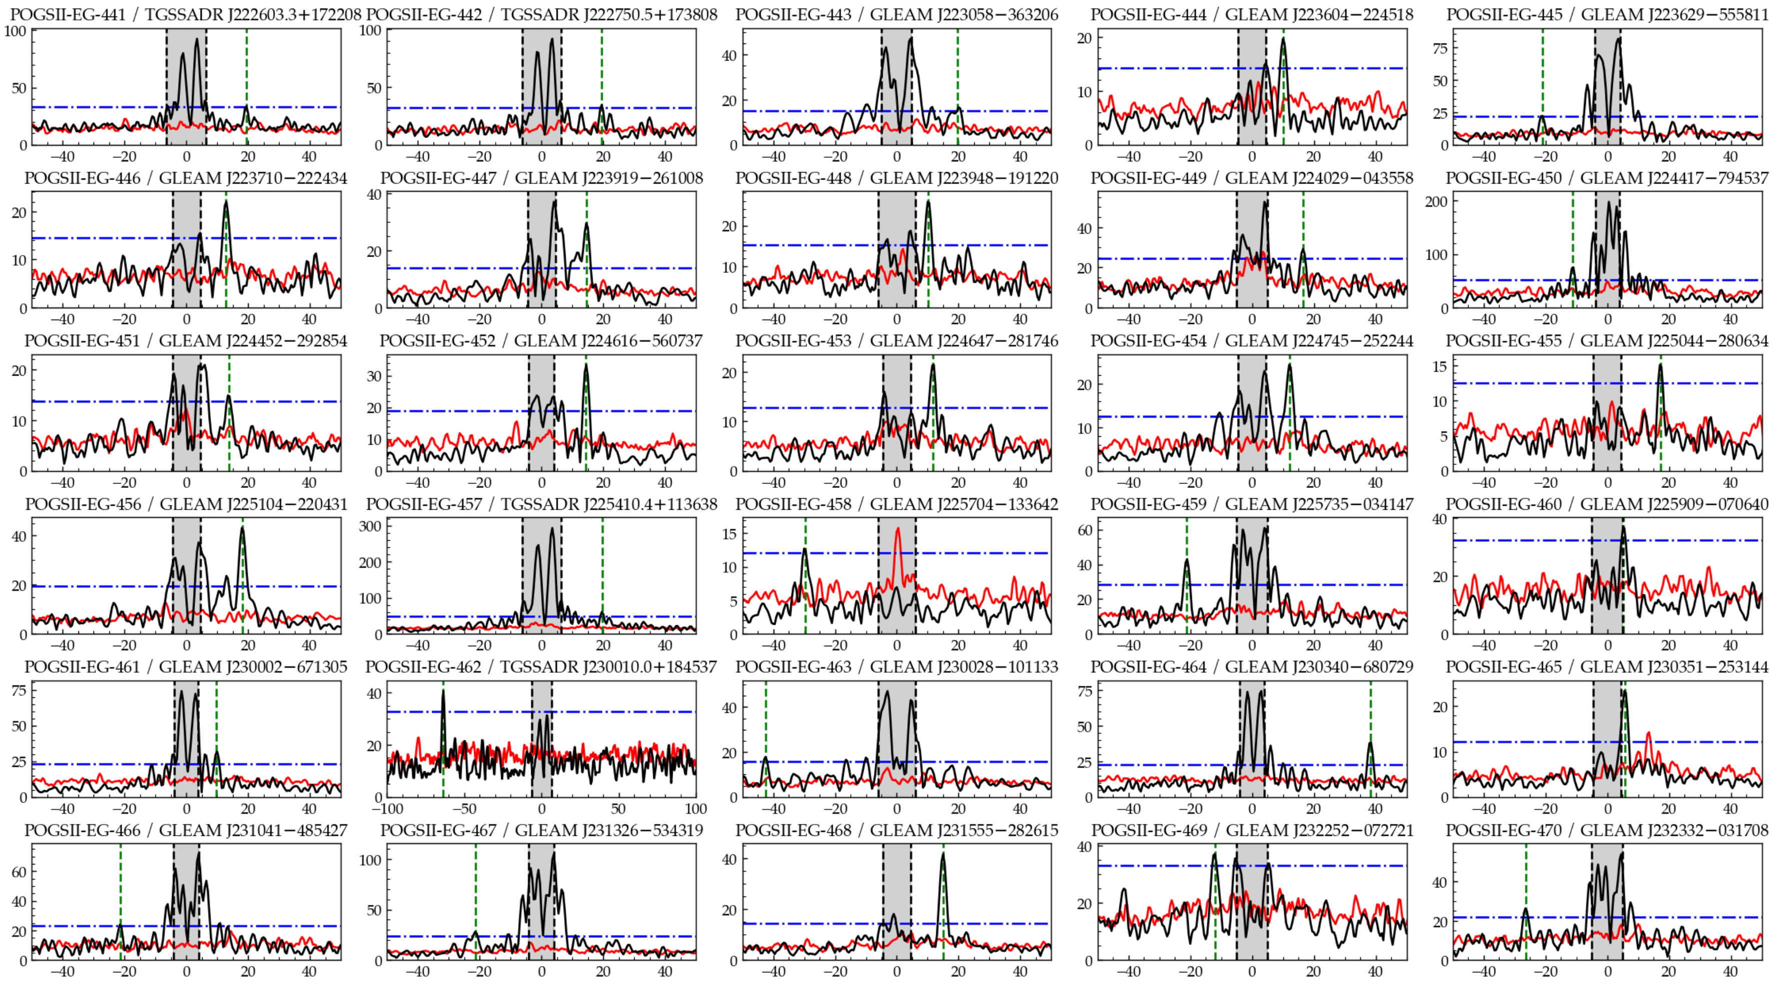


**Figure D1.** (*continued*)

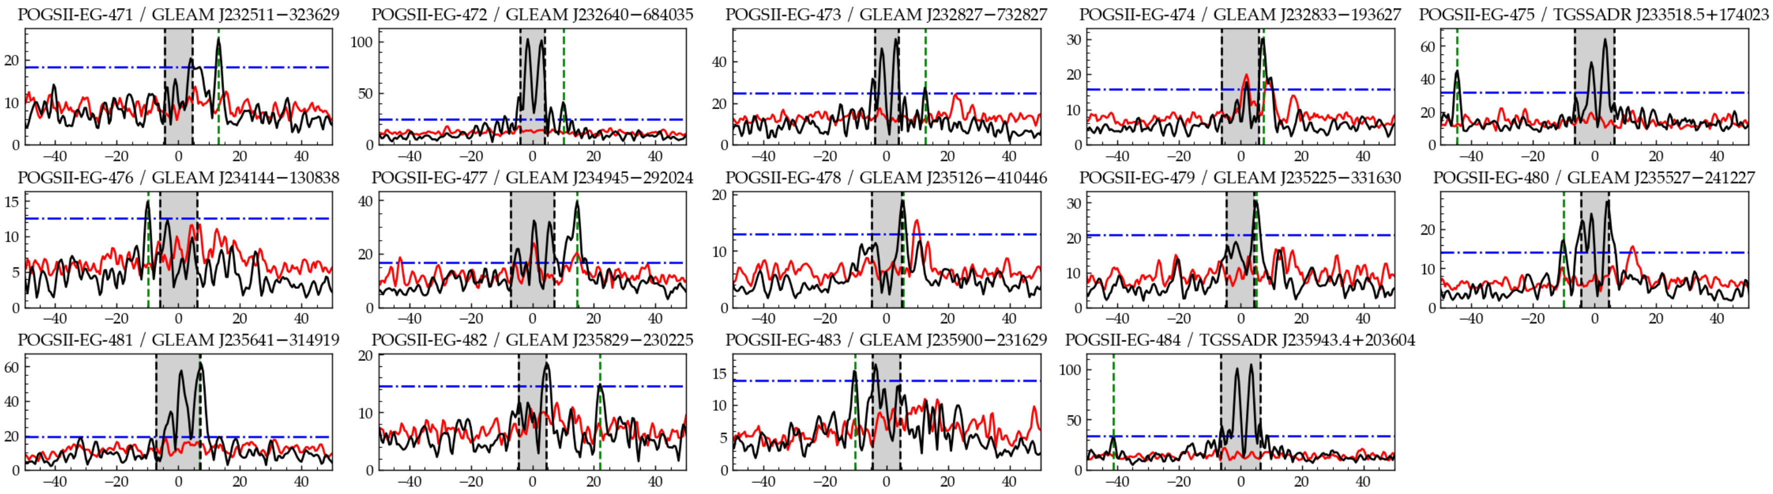


**Figure D1.** (*continued*)
